# Supplementary material for: EgoWAM: World Action Models Beyond Pixels with In-the-Wild Egocentric Human Data
Source: arXiv:2607.08436 source file (2026-10-13)
Supplement: Supplementary file 1 [file supplementary.tex]

\makeatletter
\definecolor{supptitleblue}{rgb}{0,0.08,0.45}

\newcommand*{\l@suppsec}[2]{%
  \vspace{0.32ex}%
  \noindent #1\dotfill\makebox[1.85em][r]{\textbf{#2}}\par}

\DeclareRobustCommand{\suppmark}[2]{%
  \textbf{#1}\,\textcolor{supptitleblue}{#2}}

\newcommand{\suppsection}[1]{%
  \section{#1}%
  \addcontentsline{stoc}{suppsec}{\suppmark{\thesection}{#1}}}

\newcommand*{\l@suppsubsec}[2]{%
  \vspace{0.12ex}%
  \noindent\hspace*{1.8em}#1\dotfill\makebox[1.85em][r]{#2}\par}

\DeclareRobustCommand{\suppsubmark}[2]{%
  \textcolor{supptitleblue}{#1}\hspace{0.5em}#2}

\newcommand{\suppsubsection}[1]{%
  \subsection{#1}%
  \addcontentsline{stoc}{suppsubsec}{\suppsubmark{\thesubsection}{#1}}}

\newcommand{\supptableofcontents}{%
  \begingroup
    \setlength{\parindent}{0pt}%
    \setlength{\parskip}{0pt}%
    \vspace*{0.5em}%
    \begin{center}{\LARGE\bfseries Supplementary Materials\par}\end{center}%
    \vspace{1.1em}%
    \noindent{\Large\bfseries Contents\par}%
    \vspace{0.65em}%
    \@starttoc{stoc}%
  \endgroup}
\makeatother

\appendix                 %
\setcounter{section}{0}

\supptableofcontents      %

\suppsection{Additional Real-World Experiment Results and Analysis}
\label{supp:sec:exp-analysis}

This section provides additional real-world experimental results and analysis. Further visualizations of our real-world rollouts and world-model predictions are available on our website: \url{gatech-rl2.github.io/egowam.github.io}.

\suppsubsection{Ablation on Aligned Human Data}
\label{supp:subsec:ablation-aligned-human}

\begin{wrapfigure}{r}{0.40\textwidth}
\vspace{-50pt}
\centering
\includegraphics[width=\linewidth]{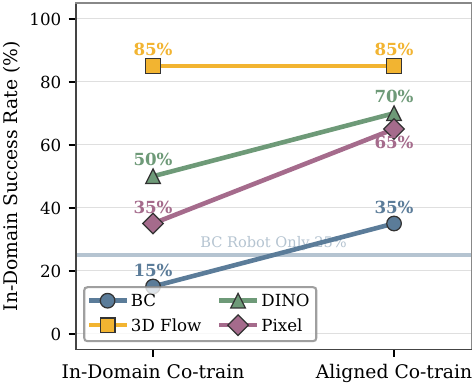}
\vspace{-18pt}
\caption{\small 
\textbf{Ablation of Aligned Human Data.} 
Aligning the demonstrator lifts BC above robot-only and gains Pixel/DINO
$20$--$30$ pts, isolating human head motion; 3D-flow holds at $85\%$ either way.
}
\label{fig:exp-ablation-aligned-human-2}
\vspace{-15pt}
\end{wrapfigure}

Sec.~\ref{subsec:exp-core-findings}\textbf{(Q3)} studied one extreme of action alignment: \emph{deliberately misaligned} human data collapses BC below its robot-only baseline, while the 3D-flow WAM stays robust. 
Here we probe the other extreme: does \emph{manually aligning} the demonstrator to the robot's viewpoint and grasp strategy (Fig.~\ref{fig:exp-setup}(c)) help each
paradigm? 
We co-train on \texttt{cup-on-saucer}, the task with the strongest human--robot mismatch (Fig.~\ref{fig:teaser}), under two $1{:}1$ human regimes:
\textbf{In-Domain Co-train} (natural human data, unmatched viewpoint and
behavior studied in Sec.~\ref{sec:experiments}) and
\textbf{Aligned Co-train} (human demonstrator intentionally mirrors the robot, described in App.~\ref{supp:sec:real-world-exp-details}).

Fig.~\ref{fig:exp-ablation-aligned-human-2} reports the difference between In-Domain Co-train and Aligned Co-train across the four variants (BC, Pixel, DINO, 3D Flow). 
Three findings stand out:
\begin{itemize}[leftmargin=*,topsep=0pt,itemsep=0pt,parsep=0pt]
    \item \textbf{Aligned human data lifts BC above its robot-only baseline.}
    BC drops under natural in-domain human data, reproducing the negative-transfer pattern. When the demonstrator is aligned to the robot, BC effectively gains from human data, confirming that BC can benefit from human data \emph{only} when the action distribution is hand-curated to match the robot's. 
    \item \textbf{Pixel and DINO improve when ego-motion is factored out at collection time.}
    Pixel rises $35\%\rightarrow65\%$ and DINO $50\%\rightarrow70\%$ when the human head motion matches the robot's static ego-camera. The gap quantifies how much these image-coordinate targets suffer when \textit{D3 (ego-motion factoring)} is violated. 
    \item \textbf{The 3D-flow WAM is invariant to alignment.} 
    It holds at $85\%$ under both regimes: the camera-stabilized 3D-flow target factors out ego-motion by construction (Sec.~\ref{subsec:world-variants}), so the gains others recover through manual alignment come for free. 
\end{itemize}

\begin{figure*}[t]
    \centering
    \includegraphics[width=\linewidth]{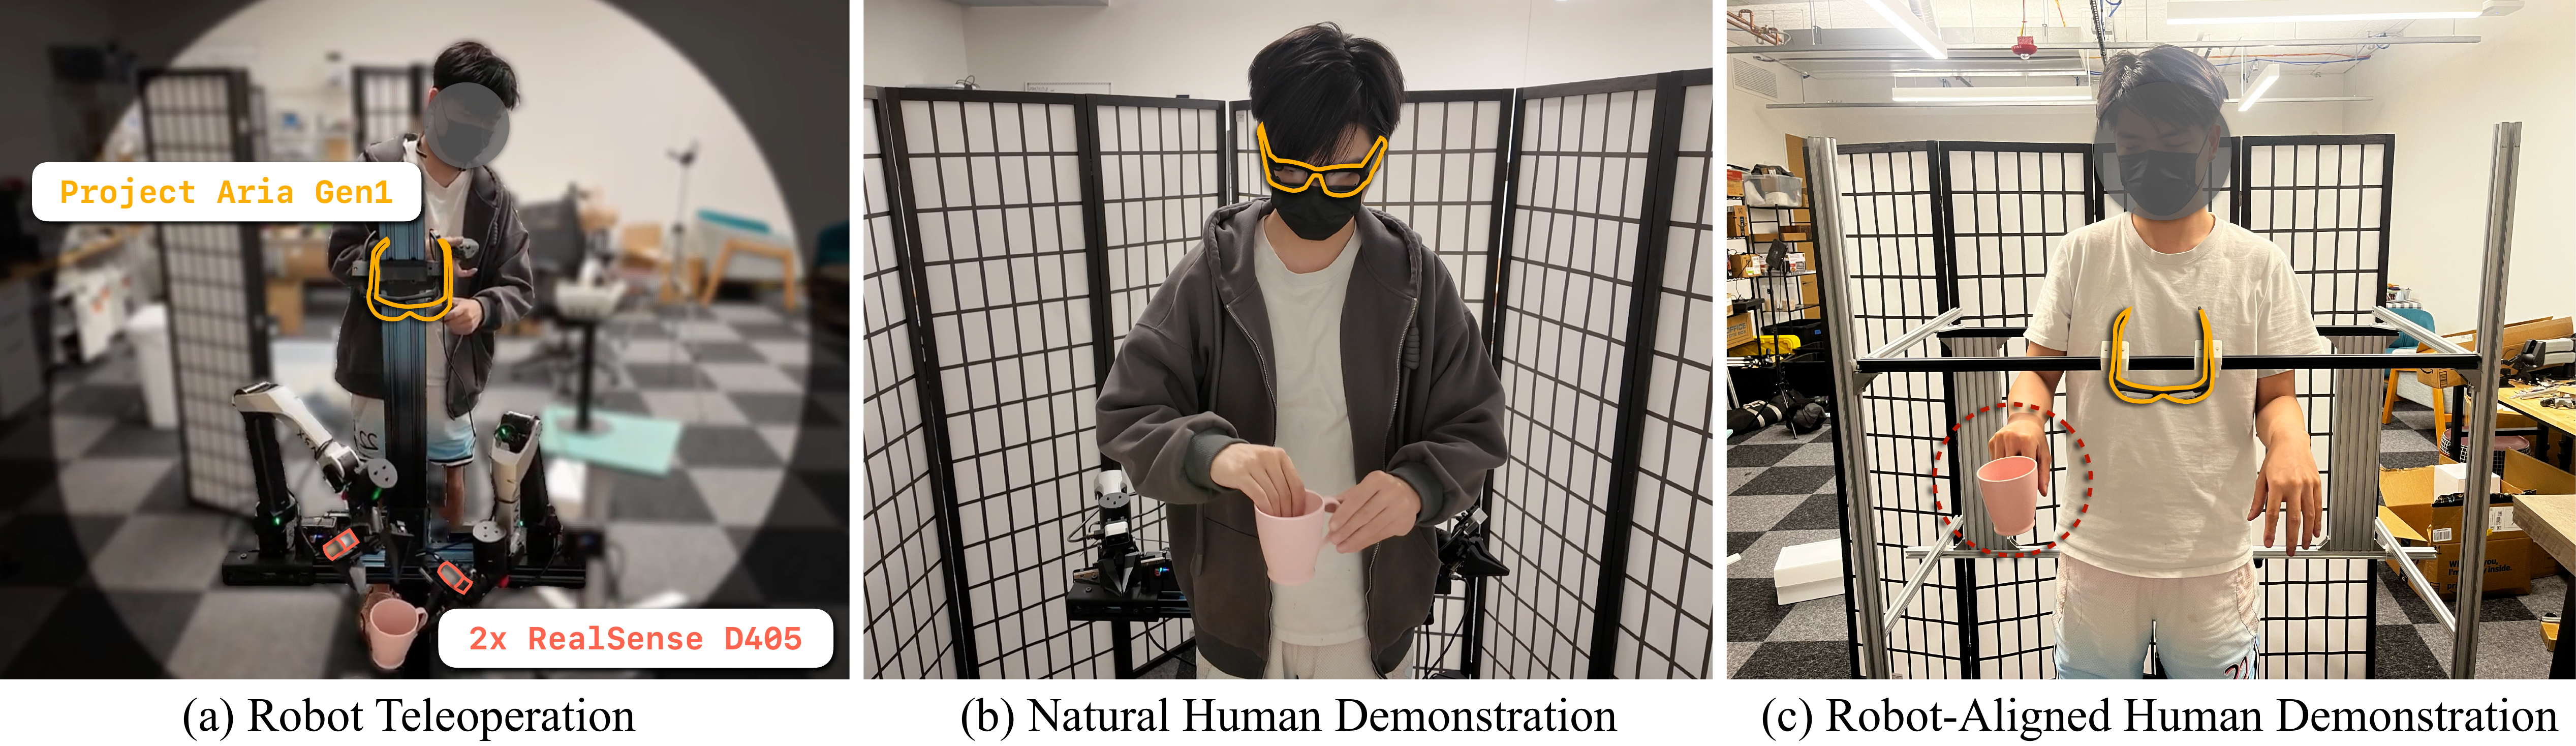}
    \vspace{-16pt}
    \caption{\small
    \textbf{Robot Platform and Data Collection.}
    \textbf{(a)} Our robot platform: two upright-mounted 6-DoF ARX5 arms with two wrist-mounted Intel RealSense D405 cameras and a head-mounted Project Aria headset, teleoperated by a human via a Meta Quest 3 interface.
    \textbf{(b)} A human wearing Project Aria glasses collects demonstrations naturally.
    \textbf{(c)} The human deliberately aligns with the robot's action, height, and viewpoint, producing a static egocentric view matched to the robot platform.
    }
    \label{fig:exp-setup}
    \vspace{-12pt}
\end{figure*}

\suppsubsection{Ablation on Human Data Modality}
\label{supp:subsec:ablation-human-modality}

\begin{wrapfigure}{r}{0.50\textwidth}
\vspace{-40pt}
\centering
\includegraphics[width=\linewidth]{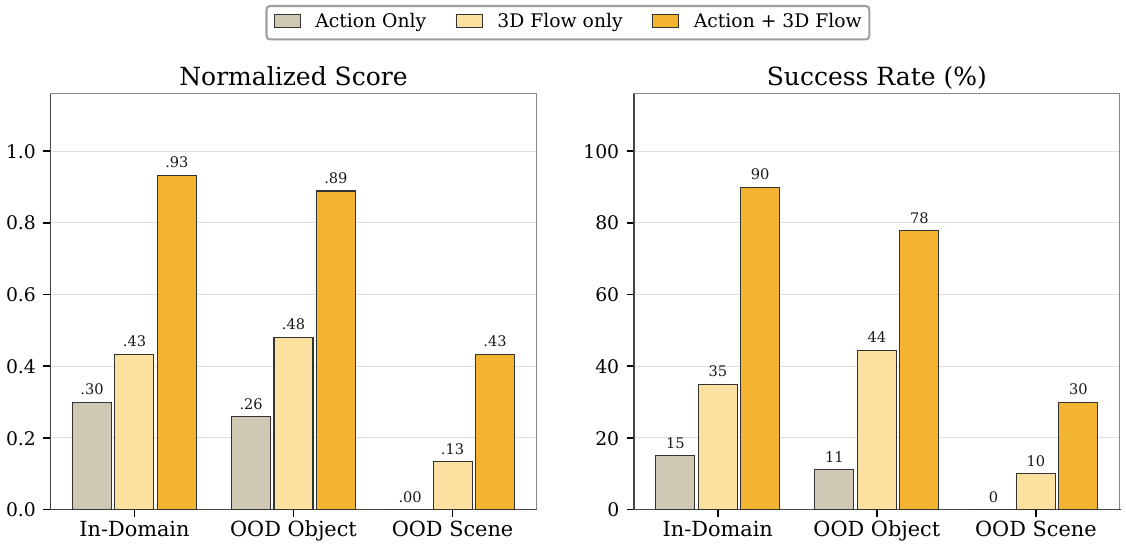}

\vspace{-10pt}
\caption{\small \textbf{Ablation of Co-Train Human Data Modality.} }
\label{fig:exp-ablation-human-modality}
\vspace{-10pt}

\end{wrapfigure}

How much of \egowam's gain comes from the \emph{action labels} on human demonstrations versus the \emph{world-model supervision}? 
We ablate three human co-training modalities on \texttt{cup-on-saucer}: \textbf{Action Only} (BC co-train baseline), \textbf{3D Flow only} (no action supervision on human batches), and \textbf{Action + 3D Flow} (full \egowam).
Fig.~\ref{fig:exp-ablation-human-modality} yields two findings:
\begin{itemize}[leftmargin=*,topsep=0pt,itemsep=0pt,parsep=0pt]
    \item \textbf{World-model supervision alone outperforms action supervision alone.} 
    3D-flow-only outperforms action-only across all three splits, most starkly on OOD~Scene, where action-only fails entirely ($0\%$) while 3D-flow-only retains $10\%$ SR. The trunk shaping induced by predicting 3D motion in human video is a stronger context-level transfer signal than action labels. 
    \item \textbf{Action labels and world-model supervision are mutually reinforcing.}
    Joint training wins on every split, and we attribute this to two complementary effects. (1) \textit{Action as context}: action labels condition the trunk on the demonstrator's intent, sharpening the world model prediction; this effect is measurable directly in the world-model loss, where co-training lowers the 3D-flow prediction loss on both the human and robot streams (Table~\ref{tab:flow_loss_modality}). (2) \textit{Action as task-relevance signal}: action labels mark which motion in the scene is task-relevant, focusing the trunk on agent-caused dynamics rather than incidental flow.
\end{itemize}
\begin{table}[h]
\centering
\caption{3D-flow world-model prediction loss. Adding action labels (\textit{Action + Flow}, full \egowam) lowers the loss over \textit{Flow-Only} on both streams, supporting \emph{action as context}.}
\label{tab:flow_loss_modality}
\begin{tabular}{lcc}
\toprule
\textbf{Flow stream} & \textbf{Flow-Only} & \textbf{Action + Flow} \\
\midrule
Human & $0.23$ & $\mathbf{0.22}$ \\
Robot & $0.20$ & $\mathbf{0.19}$ \\
\bottomrule
\end{tabular}
\end{table}

\suppsubsection{Failure Analysis for Pixel-PT on Bag-Grocery}
As shown in Fig.~\ref{fig:exp-main}, Pixel-PT (robot only) underperforms both BC and Pixel on \texttt{bag-grocery} task. Here, we provide further failure analysis on it. From our observation, most failures occurred at the bag-opening stage, and Fig.~\ref{fig:failure-pt} isolates the cause.
\textbf{Pixel-PT} renders crisp future frames in which the bag already appears open before the gripper has acted on the handles: the natural-image prior, in which bags are typically open, overrides the actual scene state, and the policy advances to the pick stage prematurely.
\textbf{Pixel (from-scratch)} produces blurrier frames but tracks bag openness faithfully, and the resulting policy opens the bag more reliably.
\textbf{Pixel-PT + EgoVerse} keeps the sharp pretrained output while predicting the closed-then-opening progression correctly, indicating that human co-training can correct noisy prior-induced hallucination in pretrained video models by increasing the data amount, and thus improves the policy a lot.
\begin{figure}
    \centering
    \includegraphics[width=\textwidth]{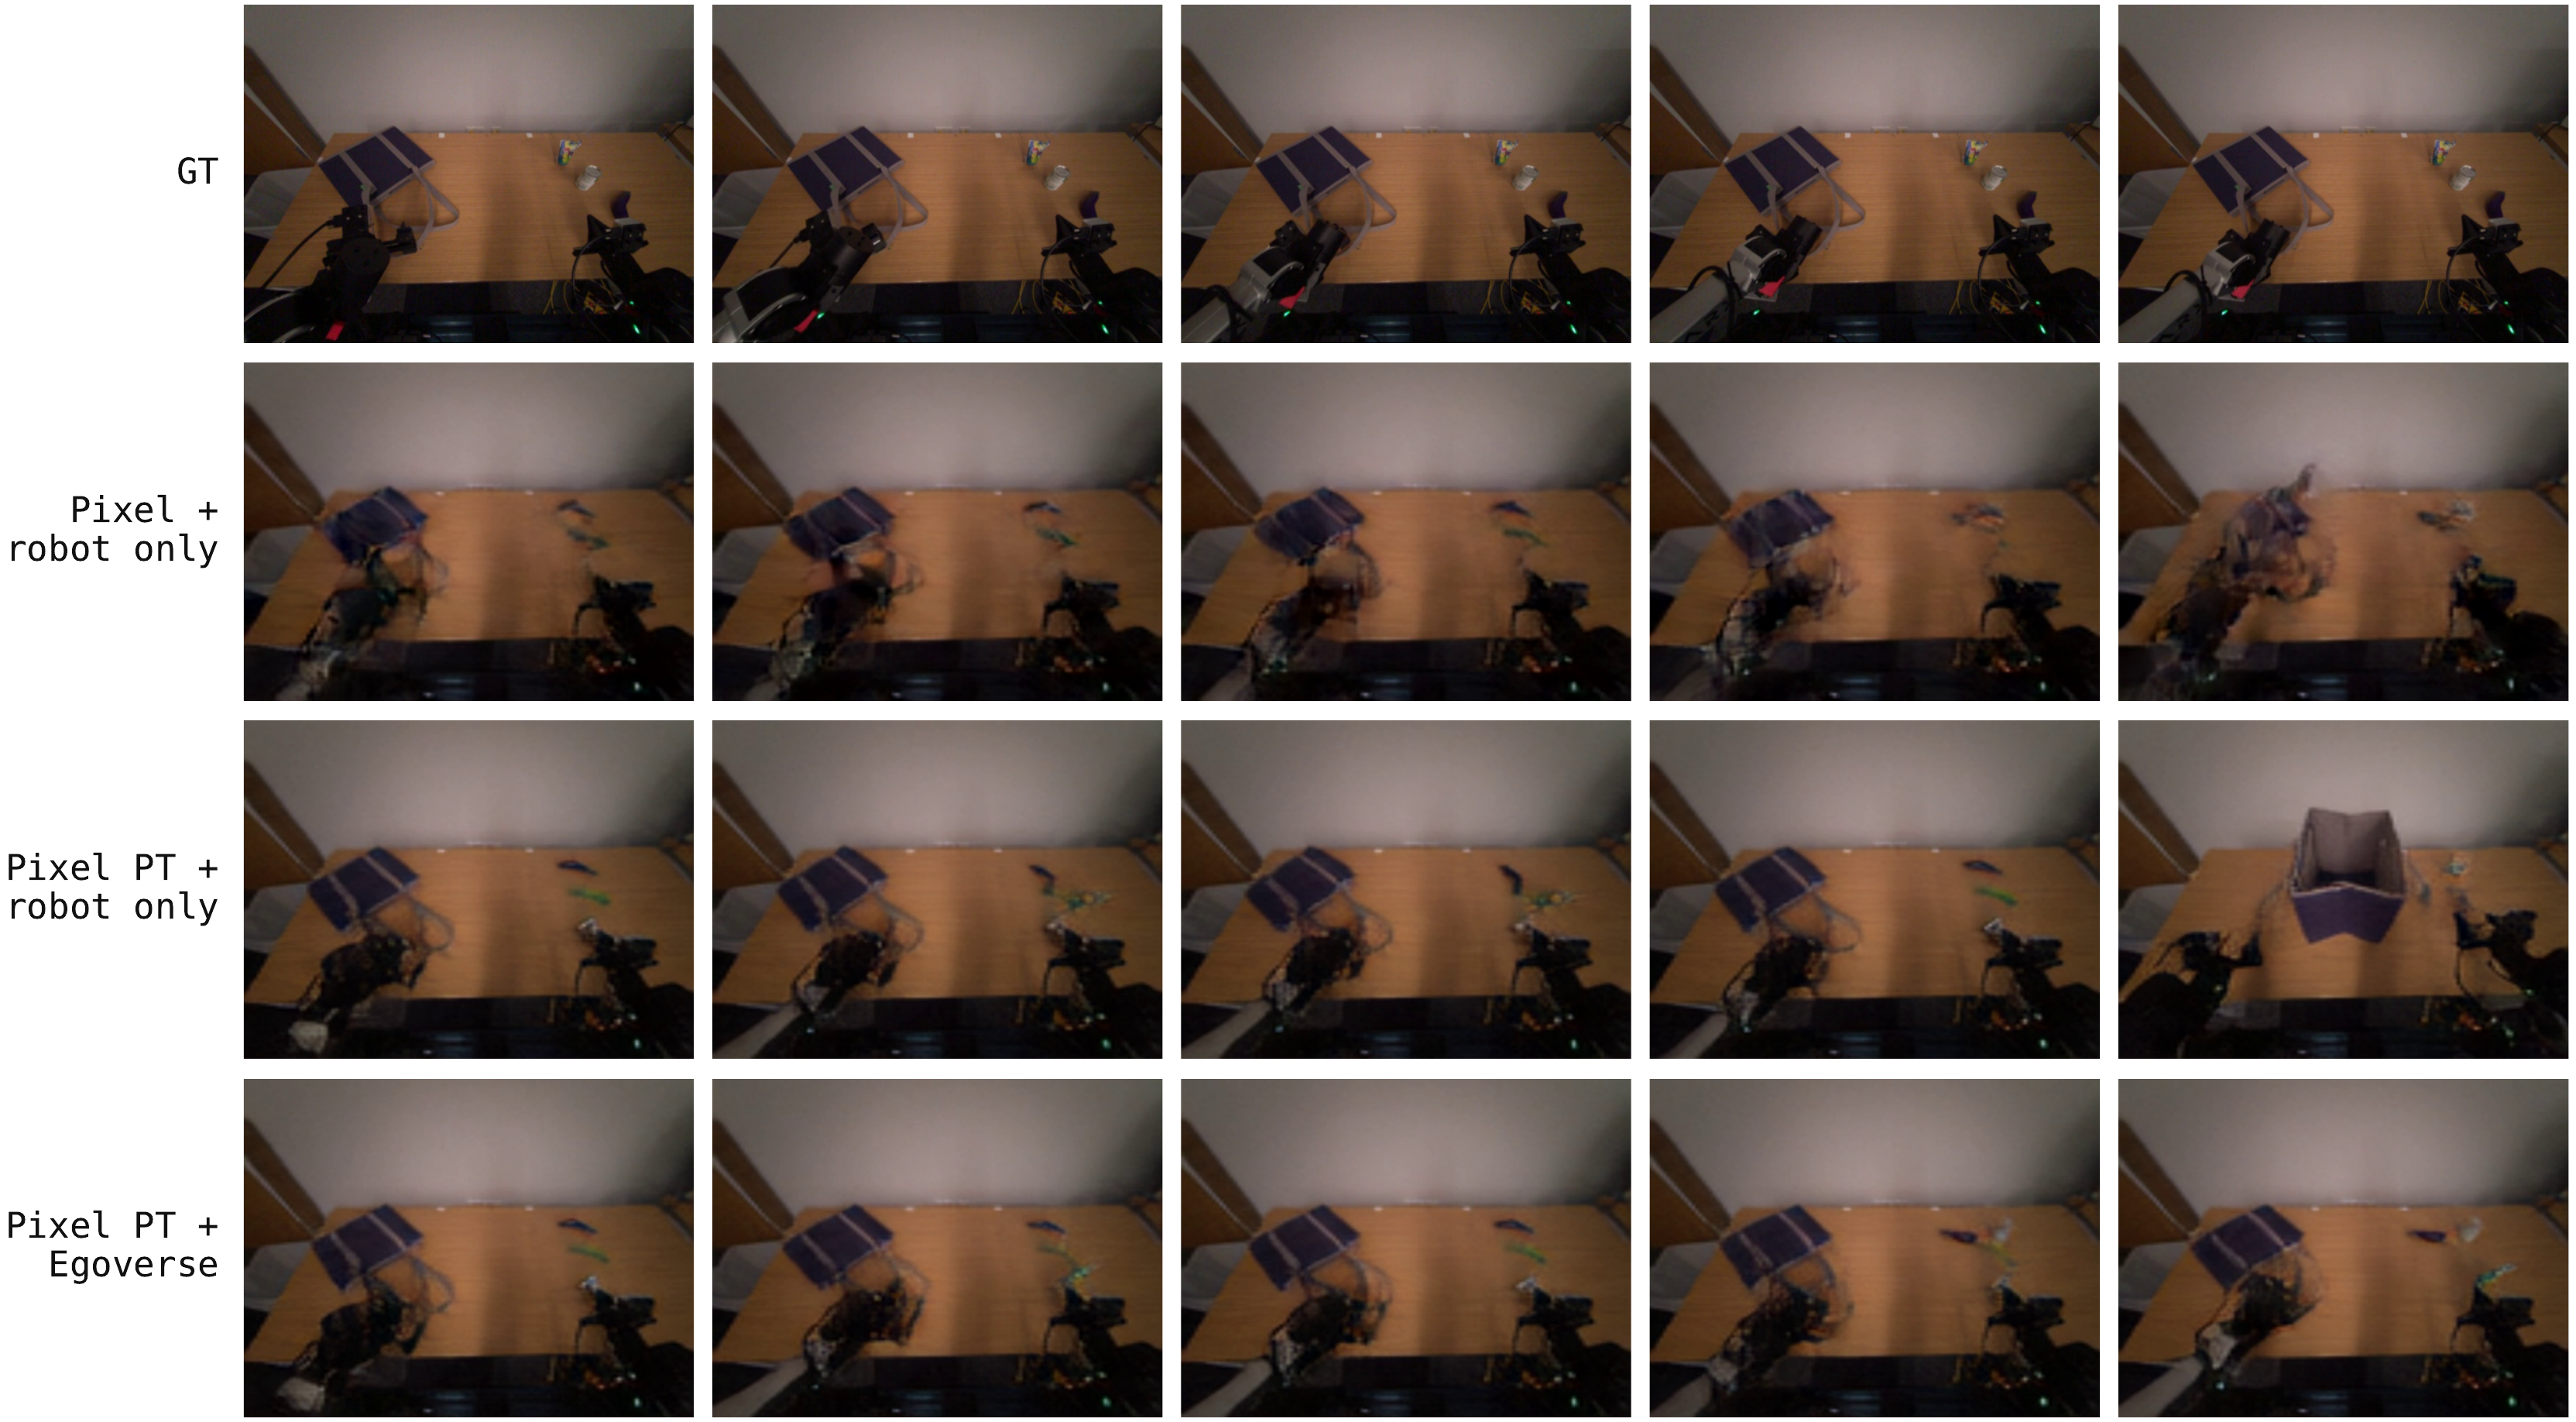}
    \vspace{-18pt}
    \caption{\small
    \textbf{Video Prediction for Failure Analysis on Bag-Grocery.}
    6-step rollouts from the same initial frame. \textbf{Pixel + robot only}: blurry but faithful, where the bag stays closed until acted on. \textbf{Pixel-PT + robot only}: hallucinates an already-open bag, causing the policy to skip the opening stage. \textbf{Pixel-PT + Egoverse}: sharp and faithful, showing human co-training removes the hallucination.
    }
    \label{fig:failure-pt}
\end{figure}

\suppsection{Additional Implementation Details}
\label{supp:sec:implement-details}

\begin{table}[t]
\centering
\caption{Hyperparameters held fixed across all world-model variants. Only the world-model head and target (bottom block) change between runs.}
\label{tab:model-parameters}
\small
\begin{tabular}{ll}
\toprule
\textbf{Component / Setting} & \textbf{Value} \\
\midrule
\multicolumn{2}{l}{\textit{Backbone and stems}} \\
Trunk (embed dim / blocks / heads) & $256 / 16 / 8$ \\
Query tokens consumed by trunk & $64$ action $+$ $16$ future (WAM); $64$ action only (BC) \\
Ego / wrist vision stem & ResNet-18~\cite{he2016resnet}, output dim $256$ \\
Proprioception stem & MLP ($14 \rightarrow 256$) \\
Cross-attn stem (latent / heads / head dim) & $16 / 8 / 64$ \\
Observation horizon & $1$ \\
Stochastic depth (drop path) & $0.1$ \\
\midrule
\multicolumn{2}{l}{\textit{Action head}} \\
Architecture & CrossTransformer (flow matching) \\
Blocks / hidden dim / heads & $6 / 128 / 4$ \\
Action dim $d_a$ & $14$ (per-arm 6-DoF $\mathrm{SE}(3)$ $+$ gripper) \\
Resampled chunk length $k$ & $100$ \\
Robot / human window $T_R, T_H$ & $1.5$\,s ($45$ frames) / $1.0$\,s ($30$ frames) \\
Prediction type / sampling steps & $v$-prediction / $50$ \\
Flow-matching $\tau$ prior & $\mathrm{Beta}(1.5, 1.0)$ \\
Normalization & quantile (1st/99th pct.\ $\rightarrow [-1, 1]$) \\
Deployment inference rate & $30$\,Hz \\
\midrule
\multicolumn{2}{l}{\textit{Optimization}} \\
Optimizer & AdamW (lr $1{\times}10^{-4}$, weight decay $1{\times}10^{-4}$) \\
Scheduler & cosine annealing ($T_{\max} = 1400$, $\eta_{\min} = 1{\times}10^{-5}$) \\
Batch size (robot / human) & $32 / 32$ \\
Steps per epoch / max epochs & $100 / 2000$ \\
Precision & bf16 \\
World-model loss weight $\lambda$ & $1.0$ \\
Augmentation (train only) & color jitter $(0.1, 0.1, 0.1, 0.05)$ \\
Image preprocessing & ImageNet normalization \\
\midrule
\multicolumn{2}{l}{\textit{World-model heads (swappable)}} \\
\textbf{Pixel:} VAE / decoder & Wan VAE~\cite{wan2025} / DiT, from scratch \\
\quad decoder (blocks / dim / heads) & $6 / 384 / 6$ \\
\quad latent ($C{\times}H{\times}W$) / input res & $16{\times}16{\times}16$ / $128$ \\
\textbf{Pixel-PT:} VAE / decoder & Wan VAE~\cite{wan2025} / VACE-1.3B~\cite{jiang2025vace}, pretrained \\
\quad decoder (layers / dim / heads / FFN) & $30 / 1536 / 12 / 8960$ \\
\quad latent ($C{\times}H{\times}W$) / input res & $16{\times}16{\times}16$ / $128$ \\
\textbf{DINO:} encoder / pre-processing & DINOv2-B~\cite{oquab2023dinov2}, frozen / drop {\tt[CLS]} \& registers, per-token LN \\
\quad denoiser ($\text{DiT}^{\text{DH}}$~\cite{zheng2025diffusiontransformersrepresentationautoencoders}) & DiT backbone $+$ wide DDT-style head~\cite{wang2025ddt} \\
\quad backbone (blocks / dim / heads) & $6 / 384 / 6$ \\
\quad wide head (blocks / dim) & $2 / 2048$ \\
\quad feature dim ($C{\times}H{\times}W$) & $768 {\times} 16 {\times} 16$ \\
\textbf{3D Flow:} tracker / denoiser & Track4World~\cite{lu2026track4world} / flow matching \\
\quad denoiser (blocks / dim / heads) & $4 / 256 / 4$ \\
\quad anchor grid / dim / horizon & $28{\times}40$ ($1120$ pts, no subsampling) / $3$ / $100$ \\
\quad query condition & anchor positions $q$ from current ego frame \\
\bottomrule
\end{tabular}
\end{table}

\suppsubsection{Behavior-Cloning Co-Training Architecture}
\label{supp:subsec:bc-cotrain}

\noindent \textbf{Stems and Trunk.}
Each embodiment is tokenized by a shallow, embodiment-specific stem that projects into a shared $256$-d space via learned query attention ($16$ latent queries, $8$ heads, head dim $64$). The egocentric stream uses a ResNet-18~\cite{he2016resnet} or pretrained DINO encoder~\cite{oquab2023dinov2, simeoni2025dinov3} stem shared across embodiments; robot batches add a matching wrist-view stem, and the $14$-d end-effector proprioception is encoded by a per-embodiment MLP. A single transformer trunk ($256$-d, $16$ blocks, $8$ heads, stochastic depth $0.1$, with learned domain embeddings) processes the observation tokens together with $64$ learnable action tokens and $16$ future tokens, using a one-frame observation history.

\noindent \textbf{Flow-Matching Action Head.}
The action head is a $6$-block CrossTransformer (hidden width $128$, $4$ heads) trained with the conditional flow-matching objective of Sec.~\ref{subsec:architecture}. It denoises a chunk of $100$ action tokens via alternating self- and cross-attention conditioned on the trunk, with the flow-matching timestep drawn from $\mathrm{Beta}(1.5,1.0)$, and is sampled with $50$ $v$-prediction steps. Cross-embodiment actions are unified to the $14$-d end-effector space and quantile-normalized (Sec.~\ref{subsec:aligned-action}).

\suppsubsection{World-Model Heads}
\label{supp:subsec:wm-head}

All three heads share the linear flow path $s^\tau=(1-\tau)\epsilon+\tau s$, $\tau\in[0,1]$, $\epsilon\sim\mathcal{N}(0,I)$, and differ only in the target $s_{t+T}$ and the head architecture that consumes the trunk embeddings.

\noindent \textbf{VAE Video Prediction Head.}
The target is the future ego frame (resized to $128{\times}128$) encoded in the latent space of a frozen pretrained Wan video VAE~\cite{wan2025}, $s = \mathrm{VAE}(I^{\text{ego}}_{t+T})$, giving a $16{\times}16{\times}16$ latent. We study two instantiations of this head, both trained under flow-matching $v$-prediction with $50$ sampling steps. \textbf{Pixel} predicts the latent with a lightweight diffusion transformer (DiT) of $6$ blocks, hidden width $384$, and $6$ heads, patchified at stride $2$ ($8{\times}8=64$ tokens) and conditioned on the mean-pooled trunk embedding, trained from scratch. \textbf{Pixel-PT} is initialized with the pretrained Wan 1.3B transformer. This backbone has 30 layers, hidden width 1536, 12 attention heads, and FFN dimension 8960. The two variants share the same VAE target and trunk conditioning, and differ in head capacity and initialization.

\noindent \textbf{RAE DINO Prediction Head.}
The target is the DINOv2-B~\cite{oquab2023dinov2} patch-feature map of the future ego frame, $s = \mathrm{DINO}\!\left(I^{\text{ego}}_{t+T}\right)$, a $16{\times}16$ token grid in $\mathbb{R}^{768}$. We adopt the Representation Autoencoder (RAE)~\cite{zheng2025diffusiontransformersrepresentationautoencoders} on two fronts: its frozen DINOv2 encoder defines the prediction target, and its $\text{DiT}^{\text{DH}}$ denoiser architecture defines our head. The trained pixel decoder is not used during \egowam training -- supervision happens directly in feature space and the world-model head is discarded at inference -- and is only invoked for visualization. Following RAE, we drop {\tt[CLS]} and register tokens and apply per-token layer normalization before the loss. The $\text{DiT}^{\text{DH}}$ head pairs a standard DiT backbone with a \emph{shallow but wide} DDT-style head~\cite{wang2025ddt}, motivated by RAE's finding that diffusion in semantic latent spaces requires denoiser width $\geq$ token dimensionality ($768$ here), below which the flow-matching loss provably fails to converge. We use a $6$-block, $384$-d backbone ($6$ heads) and a $2$-block, $2048$-d wide head, both conditioned on the mean-pooled trunk embedding, and train under $v$-prediction: $\mathcal{L}^{\mathrm{DINO}}_{\mathrm{world}} = \mathbb{E}\,\lVert\epsilon - \epsilon_{\psi}(s^{\tau},\tau,f_{\phi}(o))\rVert^{2}$, sampled with $50$ fixed Euler steps.

\noindent \textbf{3D Flow Data Processing and Prediction Head.}
The target is a dense 3D motion field over $[t,t+T]$ expressed in the camera-stabilized frame at time $t$. We obtain it with Track4World~\cite{lu2026track4world}, a feed-forward dense 3D point tracker that takes RGB frames alone and predicts per-pixel 3D scene flow together with metric depth, intrinsics, and camera poses. Raw 3D displacement on egocentric video is dominated by ego-motion: stationary objects induce large apparent flow whenever the wearer turns their head. We therefore use the Aria VIO head poses~\cite{engel2023projectarianewtool} to re-express the predicted future positions $X_{t+T}$ in the camera frame at $t$, $\tilde X_{t+T} = (T^{\text{cam}}_t)^{-1}\, T^{\text{cam}}_{t+T}\, X_{t+T}$, and define the flow target $s = F_{[t,t+T]} = \tilde X_{t+T} - X_t$. After this stabilization a static background yields near-zero flow while manipulated objects retain motion proportional to physical displacement; for robot clips the head camera is fixed, so the transform is the identity. The flow is read on a fixed $28{\times}40$ ($1120$-point) pixel-anchor grid, and to suppress tracking noise we discard anchors whose displacement falls below a movement threshold ($2$\,mm for robot tracks; $10$\,mm for human tracks, which carry residual head motion) and skip the first/last $20$ frames of each human clip. The head is a flow-matching decoder ($4$ blocks, hidden width $256$, $4$ heads) that, conditioned on the anchor positions $q$ and the trunk features, regresses the 3D displacement of \emph{all} $1120$ anchors over the $100$-step horizon (target shape $100{\times}1120{\times}3$) with no subsampling, $\mathcal{L}^{\text{Flow}}_{\text{world}} = \mathbb{E}\,\|u_\psi(s^\tau, \tau, f_\phi(o), q) - (s_q - \epsilon_q)\|^2$.

\suppsubsection{Training and Inference}
\label{supp:subsec:train-inference}

\noindent \textbf{Training.} Each step draws $32$ robot and $32$ human samples and supervises the shared trunk with $\mathcal{L}_\text{action} + \lambda\,\mathcal{L}_\text{world}$, $\lambda = 1$ (Eq.~\ref{eq:egowam-loss}). We optimize with AdamW (learning rate $1{\times}10^{-4}$, weight decay $1{\times}10^{-4}$) under cosine annealing ($T_{\max} = 1400$, $\eta_{\min} = 1{\times}10^{-5}$) in bf16. All variants except Pixel-PT are trained on a \textbf{single NVIDIA L40S GPU} for $2000$ epochs of $100$ steps; Pixel-PT is trained on $2{\times}$ L40S in data-parallel for $1000$ epochs of $100$ steps to accommodate the $1.3$B-parameter pretrained backbone within memory. Under either configuration, end-to-end training takes approximately two days per task per method. Images are ImageNet-normalized at train and test time, with color jitter ($\pm 0.1$ brightness/contrast/saturation, $\pm 0.05$ hue) added during training only. Remaining settings are listed in Table~\ref{tab:model-parameters}.

\noindent \textbf{Inference.} At deployment the world-model head $g_\psi$ is frozen and detached from the computation graph: only the shared trunk $f_\phi$ and the flow-matching action head $\pi_\theta$ are unrolled to decode $a_{t:t+k}$ from a one-frame observation, consistent with the action-only formulation in Sec.~\ref{subsec:training-inference}. The full policy runs on a \textbf{single NVIDIA RTX 4090 GPU at $30$\,Hz}, matching the control rate of the underlying ARX5 platform. Discarding the world-model head at inference also keeps the deployment footprint identical across all four world-representation variants, so any rollout differences in Sec.~\ref{sec:experiments} reflect what each target taught the trunk during training rather than test-time compute.

\suppsection{Additional Real-World Experiment Details}
\label{supp:sec:real-world-exp-details}

\suppsubsection{Robot Platform and Data Collection}

\begin{wrapfigure}{r}{0.60\textwidth}
\vspace{-10pt}
\centering
\includegraphics[width=\linewidth]{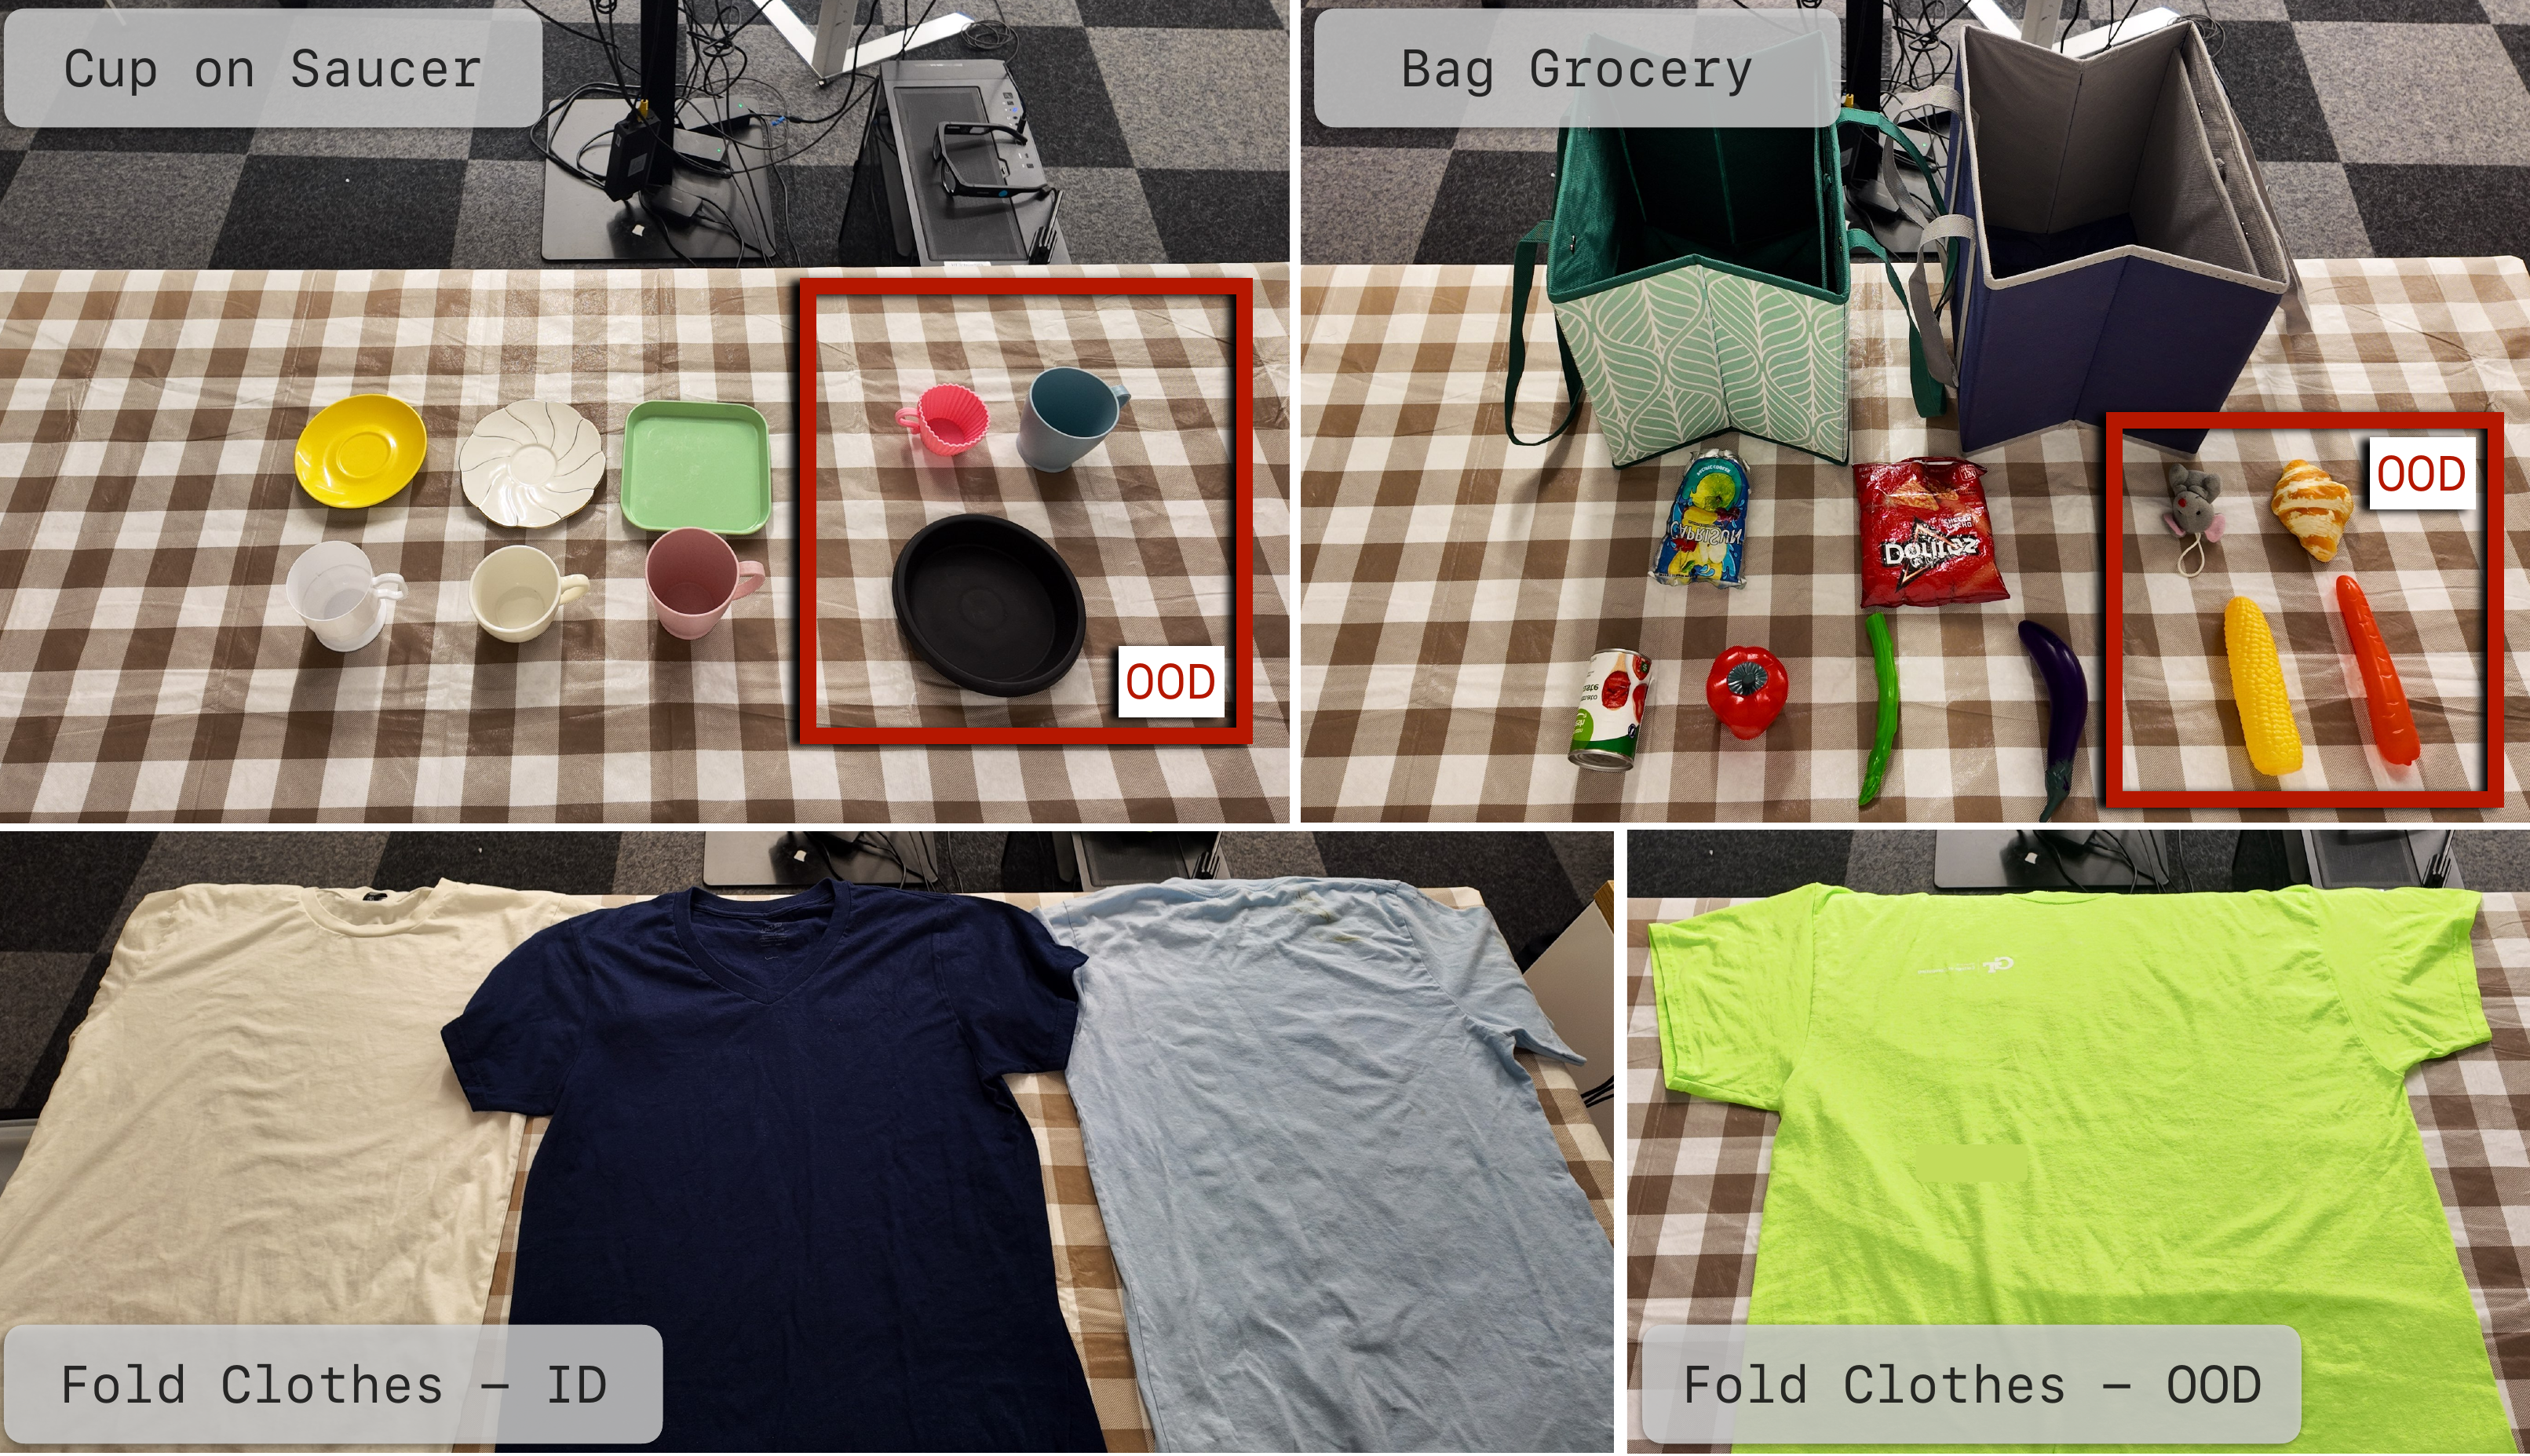}
\vspace{-18pt}
\caption{\small 
\textbf{In-Domain and OOD Objects.} 
}
\label{fig:exp-obj-set}
\vspace{-10pt}
\end{wrapfigure}

As shown in Fig.~\ref{fig:exp-setup}, our bimanual platform comprises two upright-mounted 6-DoF ARX5 arms with parallel-jaw grippers, head-mounted Project Aria Gen-1 glasses~\cite{engel2023projectarianewtool} providing the egocentric RGB stream shared with human demonstrations, and two wrist-mounted Intel RealSense D405 cameras.

We collect demonstrations through the RAIL Lab Oculus Reader~\cite{orbik2021oculusreader} interface, driving the arms with a Meta Quest~3 headset and Touch~Pro controllers. Commanded base-frame end-effector poses are converted to joint angles by the Mink IK solver~\cite{zakka2025mink}, and the resulting targets are tracked by the ARX5 joint-space controller. The runtime is a multi-threaded Python stack; low-level hardware communication runs over a CAN bus.

Robot actions are per-arm 6-DoF end-effector poses with a $1$-D gripper command, $a^{R}_{t:t+k} \in \mathbb{R}^{k \times 14}$. They are computed from commanded joint angles via forward kinematics, projected into the egocentric Aria camera frame using the calibrated extrinsics, and expressed as $(x, y, z, \text{yaw}, \text{pitch}, \text{roll})$ Euler poses per arm. Following Sec.~\ref{subsec:aligned-action}, actions are quantile-normalized by mapping each dimension's $1$st and $99$th percentiles to $[-1, 1]$ to be robust to tracking outliers.

We collect $300$–$360$ teleoperated demonstrations per task, with randomized object placements, orientations, and $4$–$8$ object combinations for each task. Per-task demonstration counts and hours are listed in Table~\ref{tab:data_composition}, and the training/testing object sets are shown in Fig.~\ref{fig:exp-obj-set}.

\begin{table}[h]
\centering
\caption{Data composition per task. \textit{In-Domain} denotes small-scale, scene- and object-aligned human data; \textit{EgoVerse} denotes the large-scale EgoVerse-A flagship split.}
\label{tab:data_composition}
\begin{tabular}{lccc}
\toprule
\textbf{Task} & \textbf{Robot} & \textbf{Human (In-Domain)} & \textbf{Human (EgoVerse)} \\
              & (\# demos / hours) & (hours) & (hours) \\
\midrule
cup-on-saucer  & 300 / 2.5h  & 2h  & 20.5h  \\
fold-clothes   & 360 / 3.0h  & 2h  & 21h  \\
bag-grocery    & 300 / 2.5h  & 2h  & 7h  \\
\bottomrule
\end{tabular}
\end{table}

\suppsubsection{Human Data Collection and EgoVerse Dataset}

\noindent \textbf{In-Domain Human Data Collection Setup.}
In-domain human data is captured with Project Aria glasses, lightweight (75~g) head-worn devices with a wide-FoV RGB camera and two synchronized monochrome scene cameras used for SLAM. Hand poses (21 keypoints and 6-DoF palm pose per hand) and a calibrated 6-DoF head pose from visual--inertial SLAM are recovered through the Aria Machine Perception Service (MPS)~\cite{engel2023projectarianewtool}. Following the EgoVerse protocol, demonstrations are recorded in roughly 5-minute units yielding several demonstrations each, within an approximately $40\,\text{cm}\times 60\,\text{cm}$ workspace with object positions randomized across trials. In-domain human data uses the \emph{same} scenes and objects as the robot data but differs in viewpoint and behavior, and is collected at a $1{:}1$ ratio with the robot demonstrations (Table~\ref{tab:data_composition}).

\noindent \textbf{Aligned and Unaligned Human Data Collection.}
To probe the robustness of each paradigm to action-(mis)aligned human data (Sec.~\ref{subsec:exp-core-findings}(Q3) and App.~\ref{supp:subsec:ablation-aligned-human}), we collect two auxiliary human datasets that bracket the alignment axis. Both reuse the in-domain human data collection setup above; only the demonstrator's execution strategy and viewpoint change.
\begin{itemize}[leftmargin=*,topsep=0pt,itemsep=0pt,parsep=0pt]
    \item \textbf{Unaligned (\texttt{bag-grocery}).} A counterfactual set in which the demonstrator performs the task in a manner whose retargeted trajectory yields \emph{inexecutable} robot actions, e.g., grasps the parallel-jaw gripper cannot reproduce (Fig.~\ref{fig:exp-ablation-aligned-human}, right). 
    \item \textbf{Aligned (\texttt{cup-on-saucer}).} The demonstrator deliberately mimics the robot's motion, with camera height and viewpoint matched to the robot's static Aria mount (Fig.~\ref{fig:exp-setup}). This isolates execution alignment from sensing alignment by collapsing the latter.
\end{itemize}

\noindent \textbf{EgoVerse Dataset.}
Our large-scale, in-the-wild human regime is the EgoVerse-A flagship split~\cite{punamiya2026egoverseegocentrichumandataset}, which spans diverse scenes, objects, and demonstrators with \emph{no} scene or object alignment to the robot data. We use the per-task flagship subsets for \texttt{cup-on-saucer}, \texttt{fold-clothes}, and \texttt{bag-grocery}, giving an overall ${\sim}10{:}1$ human-to-robot ratio (Table~\ref{tab:data_composition}). Each demonstration carries 3D hand pose for both hands (21 keypoints per hand in the camera frame) paired with a calibrated 6-DoF head pose from visual--inertial SLAM, which we use both to align the action channel and to stabilize the 3D-flow target into the camera frame at $t$ (Sec.~\ref{subsec:world-variants}).

\suppsubsection{Rollout Evaluation Protocol}

\noindent \textbf{Experiment Methods.}
Each method is evaluated on \textbf{ID} (20 rollouts: seen objects and scene, randomized positions and orientations) and \textbf{OOD} (20 rollouts: 10 unseen objects in the training scene, 10 seen objects in novel scenes with varied backgrounds and table heights), for \textbf{1800} rollouts in total across all methods and tasks. For every task we define task-specific sub-task metrics (grasps, placements, intermediate manipulations, and full completion) and report a normalized sub-task score aggregated across rollouts alongside the binary success rate. Initial conditions are randomized and held common across methods within each task to ensure a fair comparison.

\noindent \textbf{Cup-on-Saucer.}
The robot must reorient a cup from a randomized initial pose and place it upright on a saucer at a randomized position, demanding precise bimanual regrasping and fine-grained transport. Sub-task credit ($1$ point each, $3$ total) is assigned for ($i$) rotating and picking up the cup, ($ii$) a successful handover between the two arms, and ($iii$) placing the cup upright on the saucer. SR is the fraction of rollouts in which the cup is correctly placed on the saucer.

\noindent \textbf{Fold-Clothes.}
The robot must three-fold a T-shirt initialized in random configurations, a deformable task with shape variation and self-occlusion across stages. Sub-task credit ($1$ point each, $3$ total) is assigned for ($i$) the bottom-sleeves fold, ($ii$) the top-sleeves fold, and ($iii$) the final fold in half. SR requires all three stages to complete cleanly.

\noindent \textbf{Bag-Grocery.}
The robot must open a grocery bag and load three items into it from randomized positions---a long-horizon task in which the two arms first grasp the handles to open the bag, then insert items one by one. Sub-task credit is $1$ point for opening the bag and $1$ point per item placed inside, for a maximum of $4$ points per rollout; an insertion counts only if the objects are placed in left-to-right order inside the bag. SR requires all three items loaded under the ordering constraint. Because its pick-and-place motions are naturally aligned between human and robot, this is the one task where action-level co-training helps, which we exploit in the Sec.~\ref{subsec:exp-core-findings}(Q3) ablation.

\suppsection{Robot-to-Robot Transfer in Simulation: RoboTwin}
\label{supp:sec:sim}

Our real-world experiments (Sec.~\ref{sec:experiments}) establish \egowam's two central claims: that
cross-embodiment co-training transfers across the human--robot gap, and that the world-model head is
the interface that drives this transfer. To validate the same claims in a \emph{public, reproducible,
robot-to-robot} setting, we instantiate \egowam on the RoboTwin~2.0 bimanual
benchmark~\cite{chen2025robotwin2}, which ships teleoperated demonstrations for multiple robots on the
same tasks. The goal here is not a new benchmark result but a controlled replication: under a shared,
dimension-invariant end-effector action space, does cross-embodiment co-training still beat
single-embodiment training, and does the world-model head still help to transfer with abstraction?

\suppsubsection{Simulation Setup}
\label{supp:subsec:rt-setup}
RoboTwin~2.0 runs on SAPIEN~\cite{xiang2020sapien}. We use the bimanual \texttt{aloha-agilex} (two
$6$-DoF arms) as the primary embodiment and \texttt{arx-x5}, \texttt{franka}, \texttt{ur5} as
co-training embodiments, where \texttt{franka} and \texttt{ur5} are two $7$-DoF arms, on three hard tasks: \texttt{pick-diverse-bottles} ($15$-instance bottle pool),
\texttt{stack-bowls-three} (long-horizon manipulation), and \texttt{hanging-mug} (fine-grained manipulation). Each uses the shipped \texttt{demo\_clean-50}
split.

\suppsubsection{Integration and Baselines}
\label{supp:subsec:rt-integration}
We add each robot to the tokenizer stack, reusing the trunk and action head. Because the arms differ
in DoF, we predict for both arms an absolute end-effector action in a head-camera frame---
$[\mathbf{p}_{xyz},\boldsymbol{\theta}_{\text{ZYX}},g]$ per arm ($14$-D)---identical across robots, so
a single action head serves every embodiment and cross-embodiment co-training is well-posed, exactly
as in our real-world formulation (Sec.~\ref{subsec:aligned-action}). At test time the predicted chunk
is resampled to the control rate and streamed to a differential-IK controller~\cite{zakka2025mink}
under a receding horizon. Per task we train every world-model variant \emph{single}
(\texttt{aloha-agilex} only) and \emph{cross} (all four robots), holding trunk, head, and optimizer
fixed. As same-action-space references we adapt RoboTwin's official ACT~\cite{zhao2023act} and
Diffusion~Policy~\cite{chi2023diffusion} pipelines to our setting (\textbf{ACT-EE} and
\textbf{DP-EE}) by replacing their native joint-space state and action with the same $14$-D EE vector
and evaluating through the identical IK executor; they are single-embodiment and world-model-free, so
they isolate what cross-embodiment co-training and the world head add on top of the action space
alone. We evaluate all methods on $100$ held-out seeds ($\geq\!10^5$, sparse success, identical across
methods).

\suppsubsection{Results and Analysis}
\label{supp:subsec:rt-results}

\begin{table}[h]
\centering
\caption{RoboTwin held-out closed-loop success (\%, $100$ seeds). \textbf{Left:} same-action-space,
single-embodiment references (ACT-EE, DP-EE). \textbf{Right:} \egowam variants, each trained single
(\emph{s}) and cross-embodiment (\emph{c}), sharing the trunk and end-effector action head and
differing only in the world target. Best per task in \textbf{bold}. $^{\dagger}$\texttt{stack} is
evaluated on an appearance-shifted object (see text).}
\label{tab:robotwin_variants}
\setlength{\tabcolsep}{4.5pt}
\begin{tabular}{lcc@{\hskip 1.2em}cccccccc}
\toprule
& \multicolumn{2}{c}{\textbf{Baselines}} & \multicolumn{2}{c}{\textbf{BC}} &
\multicolumn{2}{c}{\textbf{Pixel}} & \multicolumn{2}{c}{\textbf{DINO}} & \multicolumn{2}{c}{\textbf{3D~Flow}} \\
\cmidrule(lr){2-3}\cmidrule(lr){4-5}\cmidrule(lr){6-7}\cmidrule(lr){8-9}\cmidrule(lr){10-11}
\textbf{Task} & ACT-EE & DP-EE & s & c & s & c & s & c & s & c \\
\midrule
\texttt{pick-diverse-bottles}          & $2$ & $5$ & $2$ & $6$ & $7$ & $11$ & $4$ & $\mathbf{28}$ & $0$ & $16$ \\
\texttt{stack-bowls-three}$^{\dagger}$  & $0$ & $0$ & $0$ & $0$ & $0$ & $0$  & $0$ & $8$  & $0$ & $\mathbf{16}$ \\
\texttt{hanging-mug}                   & $0$ & $0$ & $0$ & $0$ & $0$ & $\mathbf{1}$  & $0$ & $0$  & $0$ & $0$ \\
\bottomrule
\end{tabular}
\end{table}

Table~\ref{tab:robotwin_variants} reproduces the main paper's findings in robot-to-robot simulation.
Four points stand out:
\begin{itemize}[leftmargin=*,topsep=0pt,itemsep=0pt,parsep=0pt]
    \item \textbf{Cross-embodiment co-training beats single-embodiment training.}
    Every \egowam variant improves from single to cross (DINO $4\!\to\!28$, Pixel $7\!\to\!11$,
    BC $2\!\to\!6$ on \texttt{pick}), and cross is the \emph{only} setting that succeeds at all on
    \texttt{stack}. Since single-embodiment policies already overfit their training scenes yet barely generalize, the gap is genuine cross-embodiment transfer
    rather than better fitting, the same mechanism as our real-world results
    (Sec.~\ref{sec:experiments}).
    \item \textbf{The world-model head, not the action space, drives the transfer.}
    Under cross-embodiment training the world-model variants (Pixel/DINO/3D~Flow) consistently exceed
    the action-only BC policy. The same-action-space but world-model-free references ACT-EE/DP-EE stay
    at or below the single-embodiment variants ($\leq\!5\%$ on \texttt{pick}, $0\%$ elsewhere); since
    they change only the policy architecture, the gain is attributable to co-training through the
    world-model interface.
    \item \textbf{DINO and 3D~Flow are strong at object generalization on the first two tasks.}
    Both \texttt{pick} and \texttt{stack} stress object generalization, and the appearance-abstracting
    targets lead. On \texttt{pick} (a $15$-instance bottle pool) DINO reaches the best $28\%$ and
    3D~Flow $16\%$. On \texttt{stack}, an incidental asset change between the released demonstrations and
    the current simulator (the bowl's material shifted while its pose and geometry did not, and
    \texttt{demo\_clean} adds no texture randomization) turns evaluation into an appearance-shift test;
    \emph{only} the appearance-invariant DINO ($8\%$) and 3D~Flow ($16\%$) survive it while BC and Pixel
    collapse to $0\%$, directly reflecting the appearance-abstraction criterion~(D1) of
    Sec.~\ref{subsec:world-variants}. 
    \item \textbf{Very fine-grained manipulation still fails for all methods.}
    \texttt{hanging-mug} requires threading a mug onto a thin rack (a millimeter-precise insertion) and
    here \emph{every} method, including DINO and 3D~Flow, stays at $\leq\!1\%$. The bottleneck on this
    task is manipulation precision, not object generalization or the world target: the appearance
    abstraction that carries \texttt{pick} and \texttt{stack} does not by itself supply the
    sub-centimeter accuracy this insertion demands. Closing this gap is orthogonal to the transfer gains
    above and is left to future work.
\end{itemize}
