# Supplementary material for: EgoWAM: World Action Models Beyond Pixels with In-the-Wild Egocentric Human Data
Source: arXiv:2607.08436 source file (2026-10-13)
Supplement: Supplementary file 2 [file supp_exp_setup.tex]

\begin{figure*}[t]
    \centering
    \includegraphics[width=\linewidth]{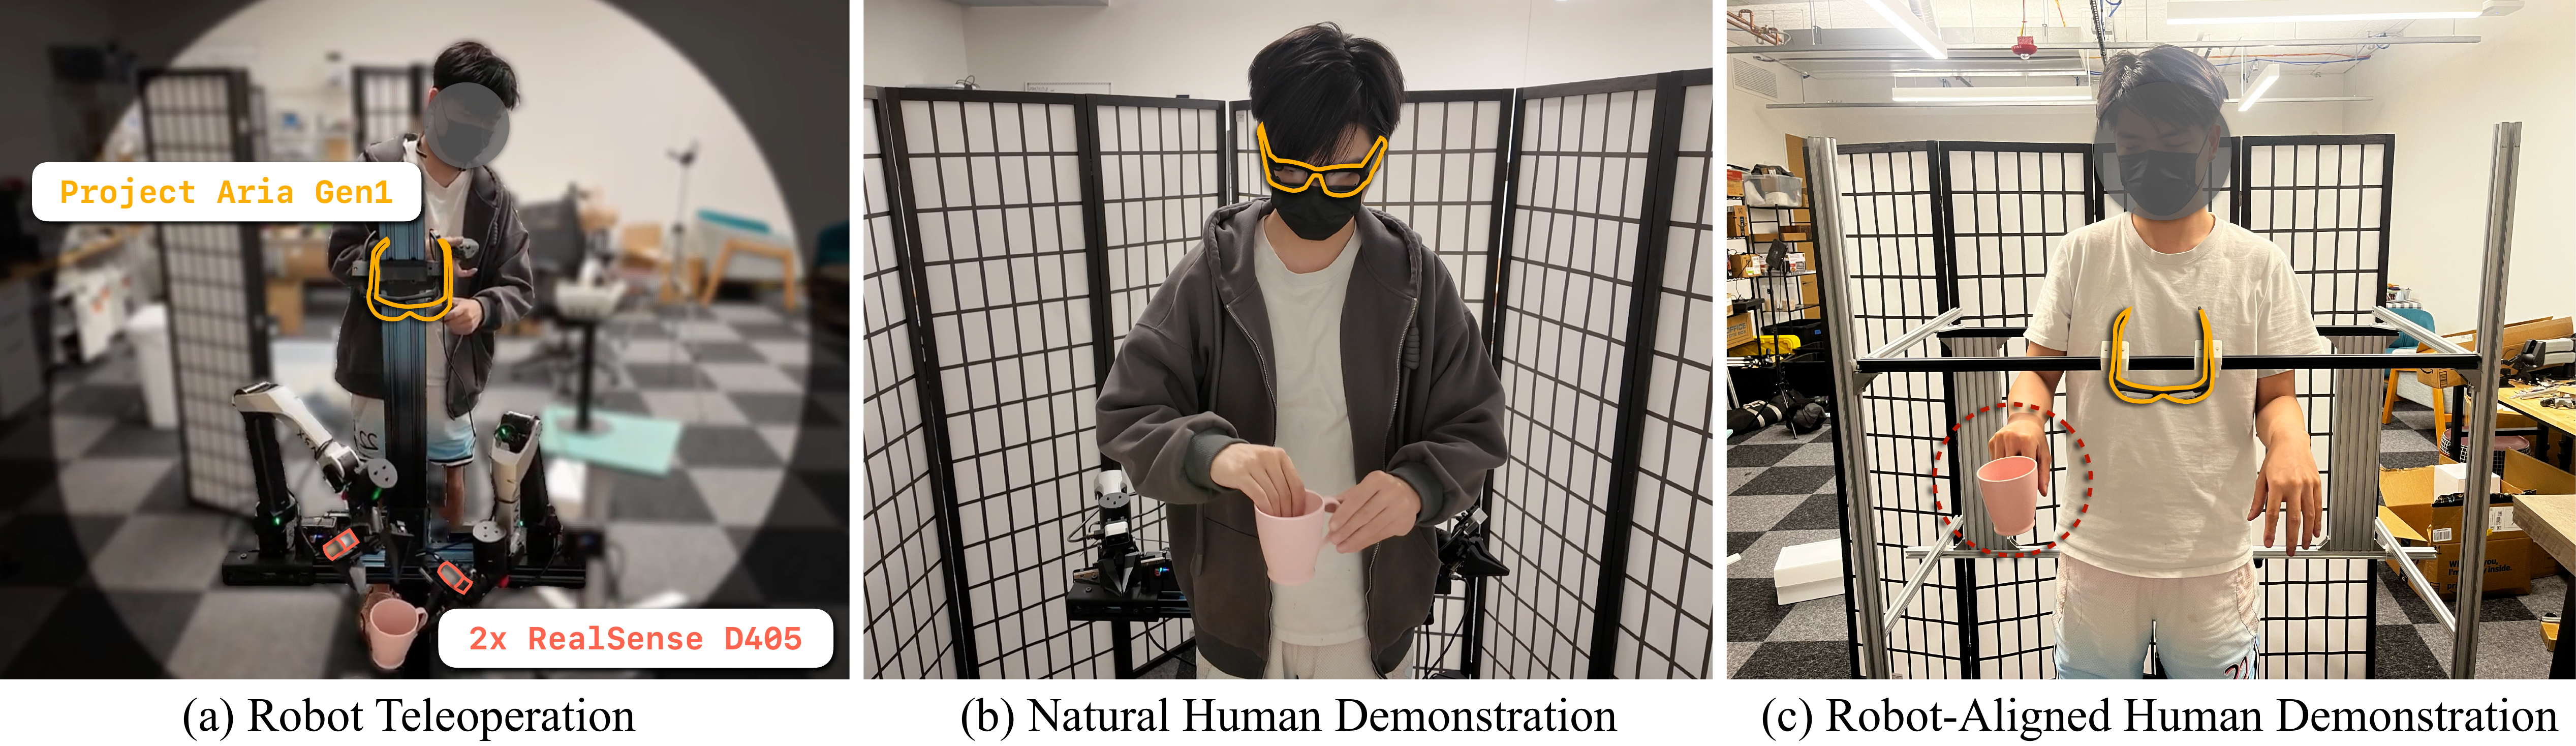}
    \vspace{-16pt}
    \caption{\small
    \textbf{Robot Platform and Data Collection.}
    \textbf{(a)} Our robot platform: two upright-mounted 6-DoF ARX5 arms with two wrist-mounted Intel RealSense D405 cameras and a head-mounted Project Aria headset, teleoperated by a human via a Meta Quest 3 interface.
    \textbf{(b)} A human wearing Project Aria glasses collects demonstrations naturally.
    \textbf{(c)} The human deliberately aligns with the robot's action, height, and viewpoint, producing a static egocentric view matched to the robot platform.
    }
    \label{fig:exp-setup}
    \vspace{-12pt}
\end{figure*}
