# Supplementary material for: EgoWAM: World Action Models Beyond Pixels with In-the-Wild Egocentric Human Data
Source: arXiv:2607.08436 source file (2026-10-13)
Supplement: Supplementary file 3 [file 001_implementation.tex]

\suppsection{Additional Implementation Details}
\label{supp:sec:implement-details}

\begin{table}[t]
\centering
\caption{Hyperparameters held fixed across all world-model variants. Only the world-model head and target (bottom block) change between runs.}
\label{tab:model-parameters}
\small
\begin{tabular}{ll}
\toprule
\textbf{Component / Setting} & \textbf{Value} \\
\midrule
\multicolumn{2}{l}{\textit{Backbone and stems}} \\
Trunk (embed dim / blocks / heads) & $256 / 16 / 8$ \\
Query tokens consumed by trunk & $64$ action $+$ $16$ future (WAM); $64$ action only (BC) \\
Ego / wrist vision stem & ResNet-18~\cite{he2016resnet}, output dim $256$ \\
Proprioception stem & MLP ($14 \rightarrow 256$) \\
Cross-attn stem (latent / heads / head dim) & $16 / 8 / 64$ \\
Observation horizon & $1$ \\
Stochastic depth (drop path) & $0.1$ \\
\midrule
\multicolumn{2}{l}{\textit{Action head}} \\
Architecture & CrossTransformer (flow matching) \\
Blocks / hidden dim / heads & $6 / 128 / 4$ \\
Action dim $d_a$ & $14$ (per-arm 6-DoF $\mathrm{SE}(3)$ $+$ gripper) \\
Resampled chunk length $k$ & $100$ \\
Robot / human window $T_R, T_H$ & $1.5$\,s ($45$ frames) / $1.0$\,s ($30$ frames) \\
Prediction type / sampling steps & $v$-prediction / $50$ \\
Flow-matching $\tau$ prior & $\mathrm{Beta}(1.5, 1.0)$ \\
Normalization & quantile (1st/99th pct.\ $\rightarrow [-1, 1]$) \\
Deployment inference rate & $30$\,Hz \\
\midrule
\multicolumn{2}{l}{\textit{Optimization}} \\
Optimizer & AdamW (lr $1{\times}10^{-4}$, weight decay $1{\times}10^{-4}$) \\
Scheduler & cosine annealing ($T_{\max} = 1400$, $\eta_{\min} = 1{\times}10^{-5}$) \\
Batch size (robot / human) & $32 / 32$ \\
Steps per epoch / max epochs & $100 / 2000$ \\
Precision & bf16 \\
World-model loss weight $\lambda$ & $1.0$ \\
Augmentation (train only) & color jitter $(0.1, 0.1, 0.1, 0.05)$ \\
Image preprocessing & ImageNet normalization \\
\midrule
\multicolumn{2}{l}{\textit{World-model heads (swappable)}} \\
\textbf{Pixel:} VAE / decoder & Wan VAE~\cite{wan2025} / DiT, from scratch \\
\quad decoder (blocks / dim / heads) & $6 / 384 / 6$ \\
\quad latent ($C{\times}H{\times}W$) / input res & $16{\times}16{\times}16$ / $128$ \\
\textbf{Pixel-PT:} VAE / decoder & Wan VAE~\cite{wan2025} / VACE-1.3B~\cite{jiang2025vace}, pretrained \\
\quad decoder (layers / dim / heads / FFN) & $30 / 1536 / 12 / 8960$ \\
\quad latent ($C{\times}H{\times}W$) / input res & $16{\times}16{\times}16$ / $128$ \\
\textbf{DINO:} encoder / pre-processing & DINOv2-B~\cite{oquab2023dinov2}, frozen / drop {\tt[CLS]} \& registers, per-token LN \\
\quad denoiser ($\text{DiT}^{\text{DH}}$~\cite{zheng2025diffusiontransformersrepresentationautoencoders}) & DiT backbone $+$ wide DDT-style head~\cite{wang2025ddt} \\
\quad backbone (blocks / dim / heads) & $6 / 384 / 6$ \\
\quad wide head (blocks / dim) & $2 / 2048$ \\
\quad feature dim ($C{\times}H{\times}W$) & $768 {\times} 16 {\times} 16$ \\
\textbf{3D Flow:} tracker / denoiser & Track4World~\cite{lu2026track4world} / flow matching \\
\quad denoiser (blocks / dim / heads) & $4 / 256 / 4$ \\
\quad anchor grid / dim / horizon & $28{\times}40$ ($1120$ pts, no subsampling) / $3$ / $100$ \\
\quad query condition & anchor positions $q$ from current ego frame \\
\bottomrule
\end{tabular}
\end{table}

\suppsubsection{Behavior-Cloning Co-Training Architecture}
\label{supp:subsec:bc-cotrain}

\noindent \textbf{Stems and Trunk.}
Each embodiment is tokenized by a shallow, embodiment-specific stem that projects into a shared $256$-d space via learned query attention ($16$ latent queries, $8$ heads, head dim $64$). The egocentric stream uses a ResNet-18~\cite{he2016resnet} or pretrained DINO encoder~\cite{oquab2023dinov2, simeoni2025dinov3} stem shared across embodiments; robot batches add a matching wrist-view stem, and the $14$-d end-effector proprioception is encoded by a per-embodiment MLP. A single transformer trunk ($256$-d, $16$ blocks, $8$ heads, stochastic depth $0.1$, with learned domain embeddings) processes the observation tokens together with $64$ learnable action tokens and $16$ future tokens, using a one-frame observation history.

\noindent \textbf{Flow-Matching Action Head.}
The action head is a $6$-block CrossTransformer (hidden width $128$, $4$ heads) trained with the conditional flow-matching objective of Sec.~\ref{subsec:architecture}. It denoises a chunk of $100$ action tokens via alternating self- and cross-attention conditioned on the trunk, with the flow-matching timestep drawn from $\mathrm{Beta}(1.5,1.0)$, and is sampled with $50$ $v$-prediction steps. Cross-embodiment actions are unified to the $14$-d end-effector space and quantile-normalized (Sec.~\ref{subsec:aligned-action}).

\suppsubsection{World-Model Heads}
\label{supp:subsec:wm-head}

All three heads share the linear flow path $s^\tau=(1-\tau)\epsilon+\tau s$, $\tau\in[0,1]$, $\epsilon\sim\mathcal{N}(0,I)$, and differ only in the target $s_{t+T}$ and the head architecture that consumes the trunk embeddings.

\noindent \textbf{VAE Video Prediction Head.}
The target is the future ego frame (resized to $128{\times}128$) encoded in the latent space of a frozen pretrained Wan video VAE~\cite{wan2025}, $s = \mathrm{VAE}(I^{\text{ego}}_{t+T})$, giving a $16{\times}16{\times}16$ latent. We study two instantiations of this head, both trained under flow-matching $v$-prediction with $50$ sampling steps. \textbf{Pixel} predicts the latent with a lightweight diffusion transformer (DiT) of $6$ blocks, hidden width $384$, and $6$ heads, patchified at stride $2$ ($8{\times}8=64$ tokens) and conditioned on the mean-pooled trunk embedding, trained from scratch. \textbf{Pixel-PT} is initialized with the pretrained Wan 1.3B transformer. This backbone has 30 layers, hidden width 1536, 12 attention heads, and FFN dimension 8960. The two variants share the same VAE target and trunk conditioning, and differ in head capacity and initialization.

\noindent \textbf{RAE DINO Prediction Head.}
The target is the DINOv2-B~\cite{oquab2023dinov2} patch-feature map of the future ego frame, $s = \mathrm{DINO}\!\left(I^{\text{ego}}_{t+T}\right)$, a $16{\times}16$ token grid in $\mathbb{R}^{768}$. We adopt the Representation Autoencoder (RAE)~\cite{zheng2025diffusiontransformersrepresentationautoencoders} on two fronts: its frozen DINOv2 encoder defines the prediction target, and its $\text{DiT}^{\text{DH}}$ denoiser architecture defines our head. The trained pixel decoder is not used during \egowam training -- supervision happens directly in feature space and the world-model head is discarded at inference -- and is only invoked for visualization. Following RAE, we drop {\tt[CLS]} and register tokens and apply per-token layer normalization before the loss. The $\text{DiT}^{\text{DH}}$ head pairs a standard DiT backbone with a \emph{shallow but wide} DDT-style head~\cite{wang2025ddt}, motivated by RAE's finding that diffusion in semantic latent spaces requires denoiser width $\geq$ token dimensionality ($768$ here), below which the flow-matching loss provably fails to converge. We use a $6$-block, $384$-d backbone ($6$ heads) and a $2$-block, $2048$-d wide head, both conditioned on the mean-pooled trunk embedding, and train under $v$-prediction: $\mathcal{L}^{\mathrm{DINO}}_{\mathrm{world}} = \mathbb{E}\,\lVert\epsilon - \epsilon_{\psi}(s^{\tau},\tau,f_{\phi}(o))\rVert^{2}$, sampled with $50$ fixed Euler steps.

\noindent \textbf{3D Flow Data Processing and Prediction Head.}
The target is a dense 3D motion field over $[t,t+T]$ expressed in the camera-stabilized frame at time $t$. We obtain it with Track4World~\cite{lu2026track4world}, a feed-forward dense 3D point tracker that takes RGB frames alone and predicts per-pixel 3D scene flow together with metric depth, intrinsics, and camera poses. Raw 3D displacement on egocentric video is dominated by ego-motion: stationary objects induce large apparent flow whenever the wearer turns their head. We therefore use the Aria VIO head poses~\cite{engel2023projectarianewtool} to re-express the predicted future positions $X_{t+T}$ in the camera frame at $t$, $\tilde X_{t+T} = (T^{\text{cam}}_t)^{-1}\, T^{\text{cam}}_{t+T}\, X_{t+T}$, and define the flow target $s = F_{[t,t+T]} = \tilde X_{t+T} - X_t$. After this stabilization a static background yields near-zero flow while manipulated objects retain motion proportional to physical displacement; for robot clips the head camera is fixed, so the transform is the identity. The flow is read on a fixed $28{\times}40$ ($1120$-point) pixel-anchor grid, and to suppress tracking noise we discard anchors whose displacement falls below a movement threshold ($2$\,mm for robot tracks; $10$\,mm for human tracks, which carry residual head motion) and skip the first/last $20$ frames of each human clip. The head is a flow-matching decoder ($4$ blocks, hidden width $256$, $4$ heads) that, conditioned on the anchor positions $q$ and the trunk features, regresses the 3D displacement of \emph{all} $1120$ anchors over the $100$-step horizon (target shape $100{\times}1120{\times}3$) with no subsampling, $\mathcal{L}^{\text{Flow}}_{\text{world}} = \mathbb{E}\,\|u_\psi(s^\tau, \tau, f_\phi(o), q) - (s_q - \epsilon_q)\|^2$.

\suppsubsection{Training and Inference}
\label{supp:subsec:train-inference}

\noindent \textbf{Training.} Each step draws $32$ robot and $32$ human samples and supervises the shared trunk with $\mathcal{L}_\text{action} + \lambda\,\mathcal{L}_\text{world}$, $\lambda = 1$ (Eq.~\ref{eq:egowam-loss}). We optimize with AdamW (learning rate $1{\times}10^{-4}$, weight decay $1{\times}10^{-4}$) under cosine annealing ($T_{\max} = 1400$, $\eta_{\min} = 1{\times}10^{-5}$) in bf16. All variants except Pixel-PT are trained on a \textbf{single NVIDIA L40S GPU} for $2000$ epochs of $100$ steps; Pixel-PT is trained on $2{\times}$ L40S in data-parallel for $1000$ epochs of $100$ steps to accommodate the $1.3$B-parameter pretrained backbone within memory. Under either configuration, end-to-end training takes approximately two days per task per method. Images are ImageNet-normalized at train and test time, with color jitter ($\pm 0.1$ brightness/contrast/saturation, $\pm 0.05$ hue) added during training only. Remaining settings are listed in Table~\ref{tab:model-parameters}.

\noindent \textbf{Inference.} At deployment the world-model head $g_\psi$ is frozen and detached from the computation graph: only the shared trunk $f_\phi$ and the flow-matching action head $\pi_\theta$ are unrolled to decode $a_{t:t+k}$ from a one-frame observation, consistent with the action-only formulation in Sec.~\ref{subsec:training-inference}. The full policy runs on a \textbf{single NVIDIA RTX 4090 GPU at $30$\,Hz}, matching the control rate of the underlying ARX5 platform. Discarding the world-model head at inference also keeps the deployment footprint identical across all four world-representation variants, so any rollout differences in Sec.~\ref{sec:experiments} reflect what each target taught the trunk during training rather than test-time compute.
