# Supplementary material for: EgoWAM: World Action Models Beyond Pixels with In-the-Wild Egocentric Human Data
Source: arXiv:2607.08436 source file (2026-10-13)
Supplement: Supplementary file 4 [file 002_exp_details.tex]

\suppsection{Additional Real-World Experiment Details}
\label{supp:sec:real-world-exp-details}

\suppsubsection{Robot Platform and Data Collection}

\begin{wrapfigure}{r}{0.60\textwidth}
\vspace{-10pt}
\centering
\includegraphics[width=\linewidth]{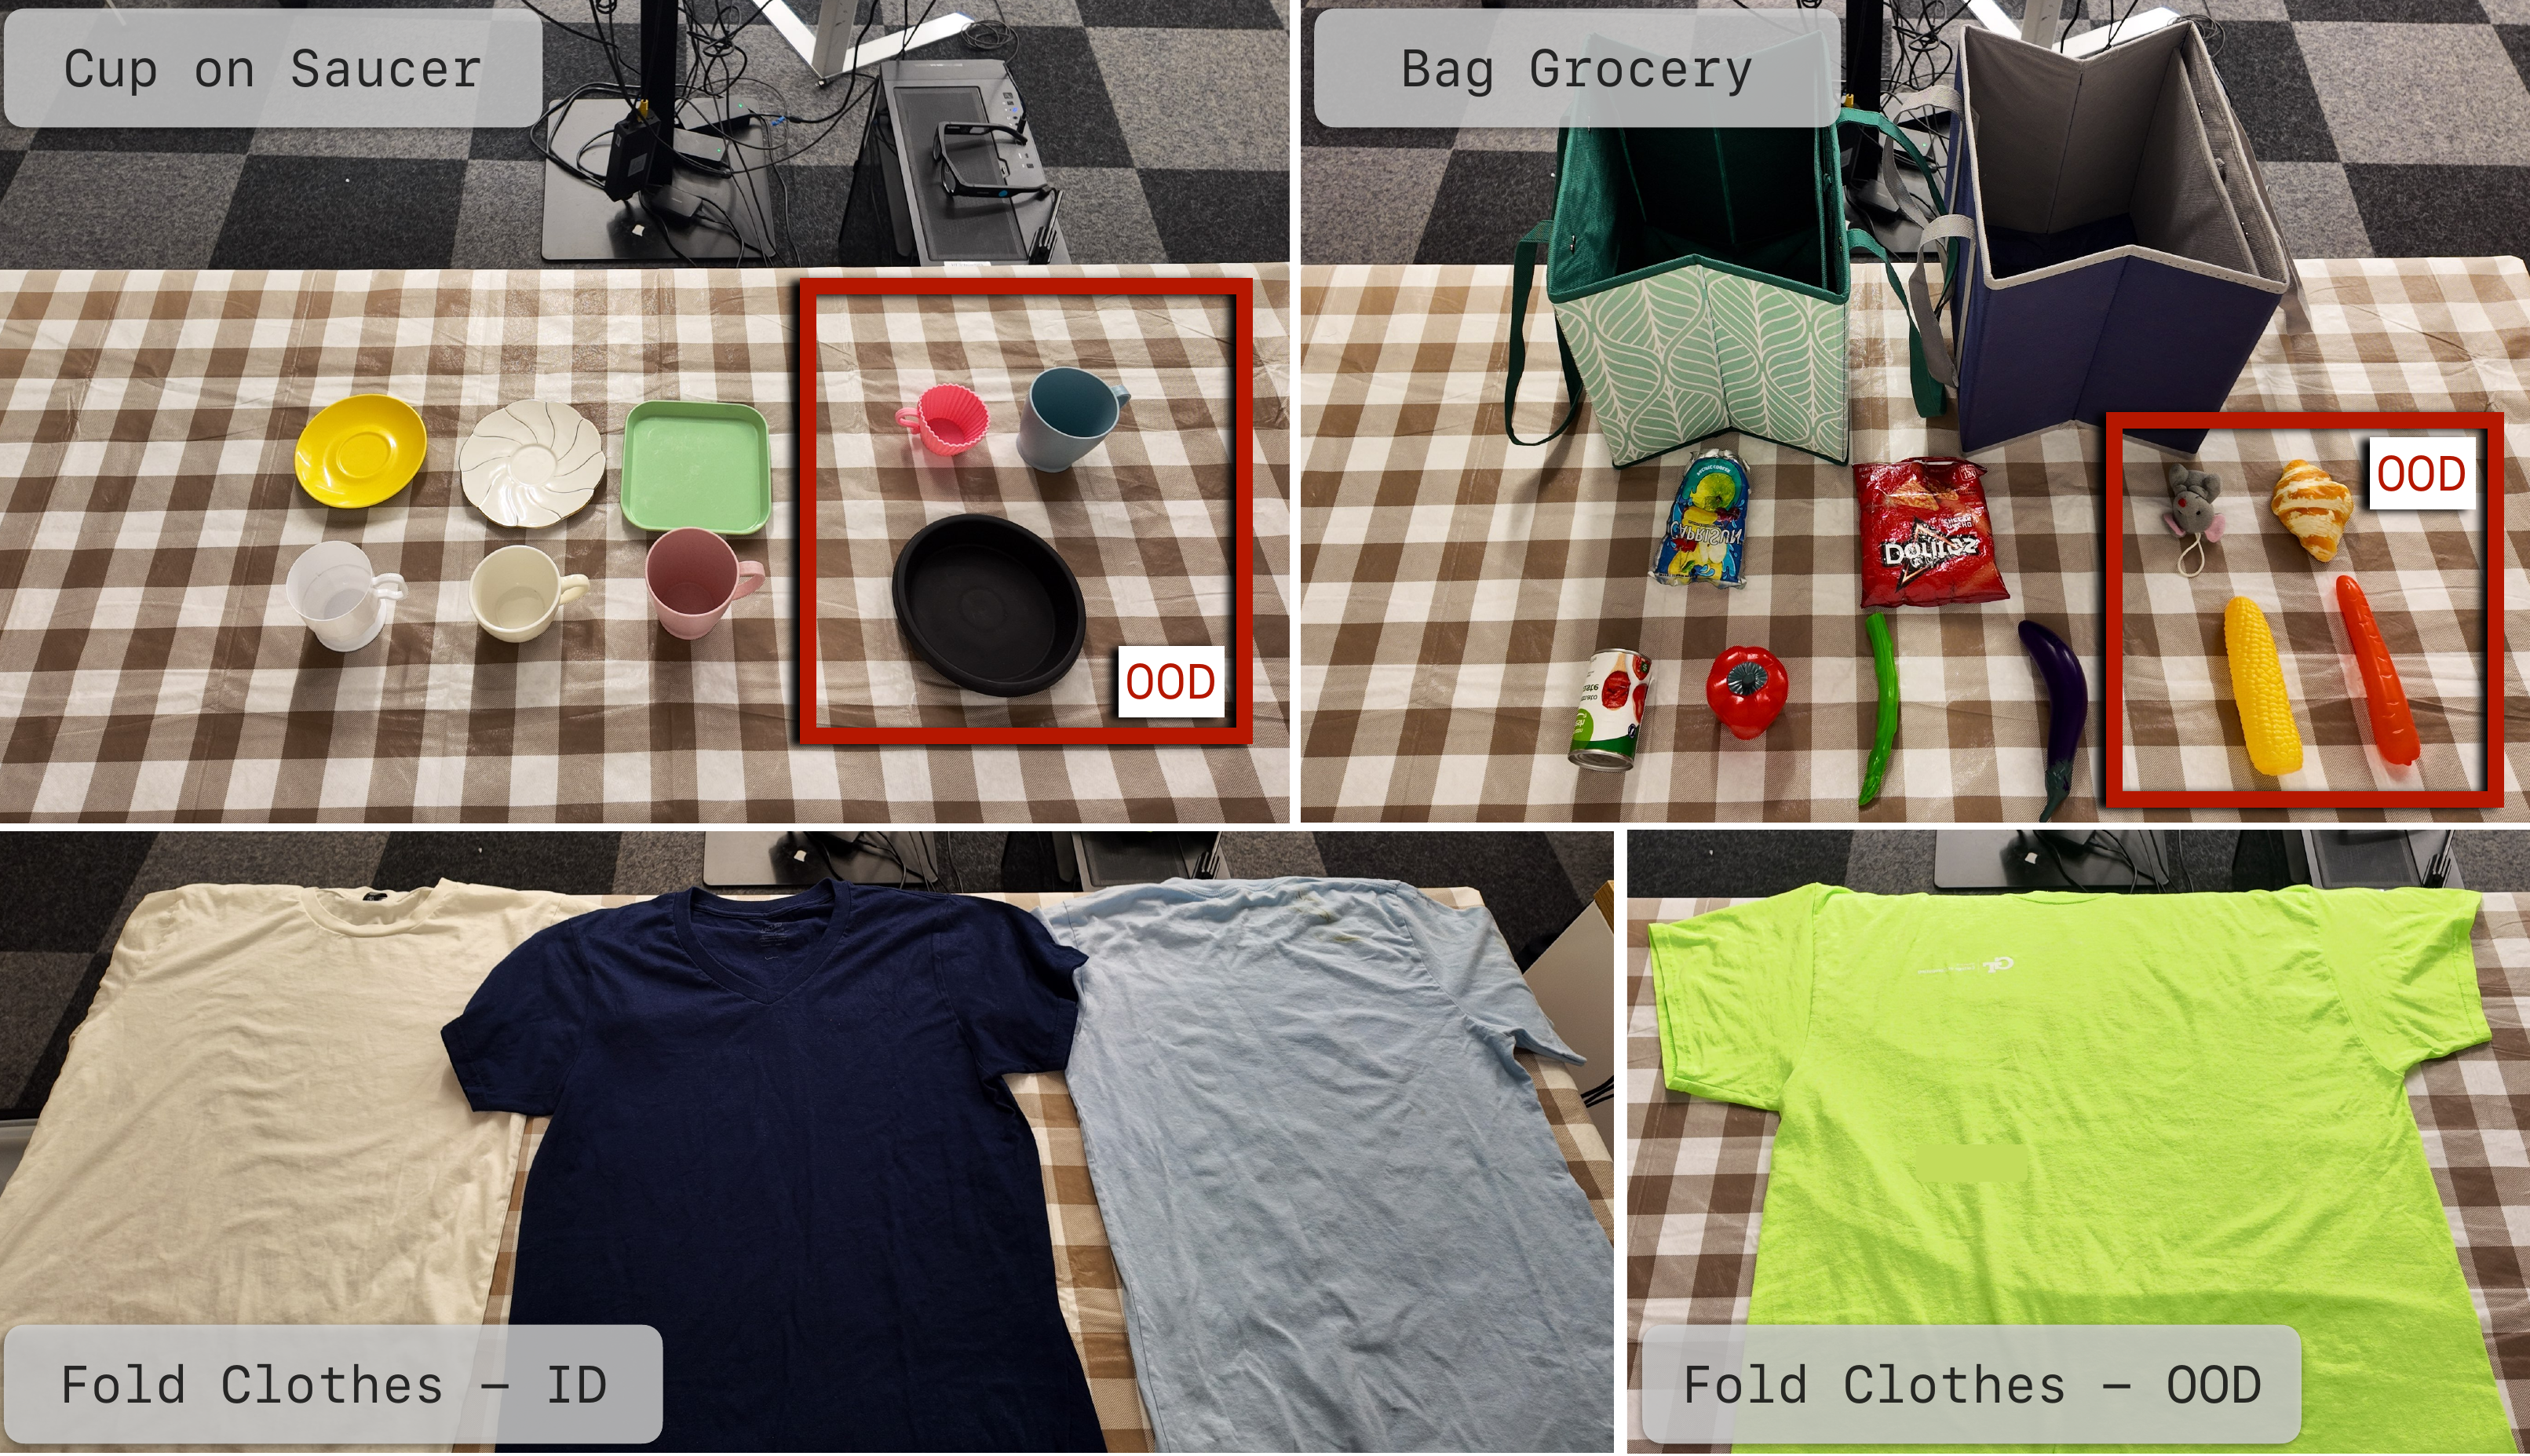}
\vspace{-18pt}
\caption{\small 
\textbf{In-Domain and OOD Objects.} 
}
\label{fig:exp-obj-set}
\vspace{-10pt}
\end{wrapfigure}

As shown in Fig.~\ref{fig:exp-setup}, our bimanual platform comprises two upright-mounted 6-DoF ARX5 arms with parallel-jaw grippers, head-mounted Project Aria Gen-1 glasses~\cite{engel2023projectarianewtool} providing the egocentric RGB stream shared with human demonstrations, and two wrist-mounted Intel RealSense D405 cameras.

We collect demonstrations through the RAIL Lab Oculus Reader~\cite{orbik2021oculusreader} interface, driving the arms with a Meta Quest~3 headset and Touch~Pro controllers. Commanded base-frame end-effector poses are converted to joint angles by the Mink IK solver~\cite{zakka2025mink}, and the resulting targets are tracked by the ARX5 joint-space controller. The runtime is a multi-threaded Python stack; low-level hardware communication runs over a CAN bus.

Robot actions are per-arm 6-DoF end-effector poses with a $1$-D gripper command, $a^{R}_{t:t+k} \in \mathbb{R}^{k \times 14}$. They are computed from commanded joint angles via forward kinematics, projected into the egocentric Aria camera frame using the calibrated extrinsics, and expressed as $(x, y, z, \text{yaw}, \text{pitch}, \text{roll})$ Euler poses per arm. Following Sec.~\ref{subsec:aligned-action}, actions are quantile-normalized by mapping each dimension's $1$st and $99$th percentiles to $[-1, 1]$ to be robust to tracking outliers.

We collect $300$–$360$ teleoperated demonstrations per task, with randomized object placements, orientations, and $4$–$8$ object combinations for each task. Per-task demonstration counts and hours are listed in Table~\ref{tab:data_composition}, and the training/testing object sets are shown in Fig.~\ref{fig:exp-obj-set}.

\begin{table}[h]
\centering
\caption{Data composition per task. \textit{In-Domain} denotes small-scale, scene- and object-aligned human data; \textit{EgoVerse} denotes the large-scale EgoVerse-A flagship split.}
\label{tab:data_composition}
\begin{tabular}{lccc}
\toprule
\textbf{Task} & \textbf{Robot} & \textbf{Human (In-Domain)} & \textbf{Human (EgoVerse)} \\
              & (\# demos / hours) & (hours) & (hours) \\
\midrule
cup-on-saucer  & 300 / 2.5h  & 2h  & 20.5h  \\
fold-clothes   & 360 / 3.0h  & 2h  & 21h  \\
bag-grocery    & 300 / 2.5h  & 2h  & 7h  \\
\bottomrule
\end{tabular}
\end{table}

\suppsubsection{Human Data Collection and EgoVerse Dataset}

\noindent \textbf{In-Domain Human Data Collection Setup.}
In-domain human data is captured with Project Aria glasses, lightweight (75~g) head-worn devices with a wide-FoV RGB camera and two synchronized monochrome scene cameras used for SLAM. Hand poses (21 keypoints and 6-DoF palm pose per hand) and a calibrated 6-DoF head pose from visual--inertial SLAM are recovered through the Aria Machine Perception Service (MPS)~\cite{engel2023projectarianewtool}. Following the EgoVerse protocol, demonstrations are recorded in roughly 5-minute units yielding several demonstrations each, within an approximately $40\,\text{cm}\times 60\,\text{cm}$ workspace with object positions randomized across trials. In-domain human data uses the \emph{same} scenes and objects as the robot data but differs in viewpoint and behavior, and is collected at a $1{:}1$ ratio with the robot demonstrations (Table~\ref{tab:data_composition}).

\noindent \textbf{Aligned and Unaligned Human Data Collection.}
To probe the robustness of each paradigm to action-(mis)aligned human data (Sec.~\ref{subsec:exp-core-findings}(Q3) and App.~\ref{supp:subsec:ablation-aligned-human}), we collect two auxiliary human datasets that bracket the alignment axis. Both reuse the in-domain human data collection setup above; only the demonstrator's execution strategy and viewpoint change.
\begin{itemize}[leftmargin=*,topsep=0pt,itemsep=0pt,parsep=0pt]
    \item \textbf{Unaligned (\texttt{bag-grocery}).} A counterfactual set in which the demonstrator performs the task in a manner whose retargeted trajectory yields \emph{inexecutable} robot actions, e.g., grasps the parallel-jaw gripper cannot reproduce (Fig.~\ref{fig:exp-ablation-aligned-human}, right). 
    \item \textbf{Aligned (\texttt{cup-on-saucer}).} The demonstrator deliberately mimics the robot's motion, with camera height and viewpoint matched to the robot's static Aria mount (Fig.~\ref{fig:exp-setup}). This isolates execution alignment from sensing alignment by collapsing the latter.
\end{itemize}

\noindent \textbf{EgoVerse Dataset.}
Our large-scale, in-the-wild human regime is the EgoVerse-A flagship split~\cite{punamiya2026egoverseegocentrichumandataset}, which spans diverse scenes, objects, and demonstrators with \emph{no} scene or object alignment to the robot data. We use the per-task flagship subsets for \texttt{cup-on-saucer}, \texttt{fold-clothes}, and \texttt{bag-grocery}, giving an overall ${\sim}10{:}1$ human-to-robot ratio (Table~\ref{tab:data_composition}). Each demonstration carries 3D hand pose for both hands (21 keypoints per hand in the camera frame) paired with a calibrated 6-DoF head pose from visual--inertial SLAM, which we use both to align the action channel and to stabilize the 3D-flow target into the camera frame at $t$ (Sec.~\ref{subsec:world-variants}).

\suppsubsection{Rollout Evaluation Protocol}

\noindent \textbf{Experiment Methods.}
Each method is evaluated on \textbf{ID} (20 rollouts: seen objects and scene, randomized positions and orientations) and \textbf{OOD} (20 rollouts: 10 unseen objects in the training scene, 10 seen objects in novel scenes with varied backgrounds and table heights), for \textbf{1800} rollouts in total across all methods and tasks. For every task we define task-specific sub-task metrics (grasps, placements, intermediate manipulations, and full completion) and report a normalized sub-task score aggregated across rollouts alongside the binary success rate. Initial conditions are randomized and held common across methods within each task to ensure a fair comparison.

\noindent \textbf{Cup-on-Saucer.}
The robot must reorient a cup from a randomized initial pose and place it upright on a saucer at a randomized position, demanding precise bimanual regrasping and fine-grained transport. Sub-task credit ($1$ point each, $3$ total) is assigned for ($i$) rotating and picking up the cup, ($ii$) a successful handover between the two arms, and ($iii$) placing the cup upright on the saucer. SR is the fraction of rollouts in which the cup is correctly placed on the saucer.

\noindent \textbf{Fold-Clothes.}
The robot must three-fold a T-shirt initialized in random configurations, a deformable task with shape variation and self-occlusion across stages. Sub-task credit ($1$ point each, $3$ total) is assigned for ($i$) the bottom-sleeves fold, ($ii$) the top-sleeves fold, and ($iii$) the final fold in half. SR requires all three stages to complete cleanly.

\noindent \textbf{Bag-Grocery.}
The robot must open a grocery bag and load three items into it from randomized positions---a long-horizon task in which the two arms first grasp the handles to open the bag, then insert items one by one. Sub-task credit is $1$ point for opening the bag and $1$ point per item placed inside, for a maximum of $4$ points per rollout; an insertion counts only if the objects are placed in left-to-right order inside the bag. SR requires all three items loaded under the ordering constraint. Because its pick-and-place motions are naturally aligned between human and robot, this is the one task where action-level co-training helps, which we exploit in the Sec.~\ref{subsec:exp-core-findings}(Q3) ablation.
