# Supplementary material for: EgoWAM: World Action Models Beyond Pixels with In-the-Wild Egocentric Human Data
Source: arXiv:2607.08436 source file (2026-10-13)
Supplement: Supplementary file 5 [file 003_exp_analysis.tex]

\suppsection{Additional Real-World Experiment Results and Analysis}
\label{supp:sec:exp-analysis}

This section provides additional real-world experimental results and analysis. Further visualizations of our real-world rollouts and world-model predictions are available on our website: \url{gatech-rl2.github.io/egowam.github.io}.

\suppsubsection{Ablation on Aligned Human Data}
\label{supp:subsec:ablation-aligned-human}

\begin{wrapfigure}{r}{0.40\textwidth}
\vspace{-50pt}
\centering
\includegraphics[width=\linewidth]{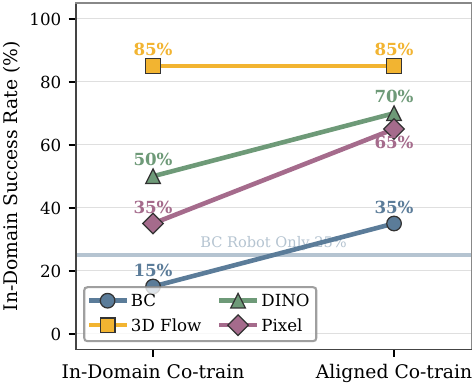}
\vspace{-18pt}
\caption{\small 
\textbf{Ablation of Aligned Human Data.} 
Aligning the demonstrator lifts BC above robot-only and gains Pixel/DINO
$20$--$30$ pts, isolating human head motion; 3D-flow holds at $85\%$ either way.
}
\label{fig:exp-ablation-aligned-human-2}
\vspace{-15pt}
\end{wrapfigure}

Sec.~\ref{subsec:exp-core-findings}\textbf{(Q3)} studied one extreme of action alignment: \emph{deliberately misaligned} human data collapses BC below its robot-only baseline, while the 3D-flow WAM stays robust. 
Here we probe the other extreme: does \emph{manually aligning} the demonstrator to the robot's viewpoint and grasp strategy (Fig.~\ref{fig:exp-setup}(c)) help each
paradigm? 
We co-train on \texttt{cup-on-saucer}, the task with the strongest human--robot mismatch (Fig.~\ref{fig:teaser}), under two $1{:}1$ human regimes:
\textbf{In-Domain Co-train} (natural human data, unmatched viewpoint and
behavior studied in Sec.~\ref{sec:experiments}) and
\textbf{Aligned Co-train} (human demonstrator intentionally mirrors the robot, described in App.~\ref{supp:sec:real-world-exp-details}).

Fig.~\ref{fig:exp-ablation-aligned-human-2} reports the difference between In-Domain Co-train and Aligned Co-train across the four variants (BC, Pixel, DINO, 3D Flow). 
Three findings stand out:
\begin{itemize}[leftmargin=*,topsep=0pt,itemsep=0pt,parsep=0pt]
    \item \textbf{Aligned human data lifts BC above its robot-only baseline.}
    BC drops under natural in-domain human data, reproducing the negative-transfer pattern. When the demonstrator is aligned to the robot, BC effectively gains from human data, confirming that BC can benefit from human data \emph{only} when the action distribution is hand-curated to match the robot's. 
    \item \textbf{Pixel and DINO improve when ego-motion is factored out at collection time.}
    Pixel rises $35\%\rightarrow65\%$ and DINO $50\%\rightarrow70\%$ when the human head motion matches the robot's static ego-camera. The gap quantifies how much these image-coordinate targets suffer when \textit{D3 (ego-motion factoring)} is violated. 
    \item \textbf{The 3D-flow WAM is invariant to alignment.} 
    It holds at $85\%$ under both regimes: the camera-stabilized 3D-flow target factors out ego-motion by construction (Sec.~\ref{subsec:world-variants}), so the gains others recover through manual alignment come for free. 
\end{itemize}

\begin{figure*}[t]
    \centering
    \includegraphics[width=\linewidth]{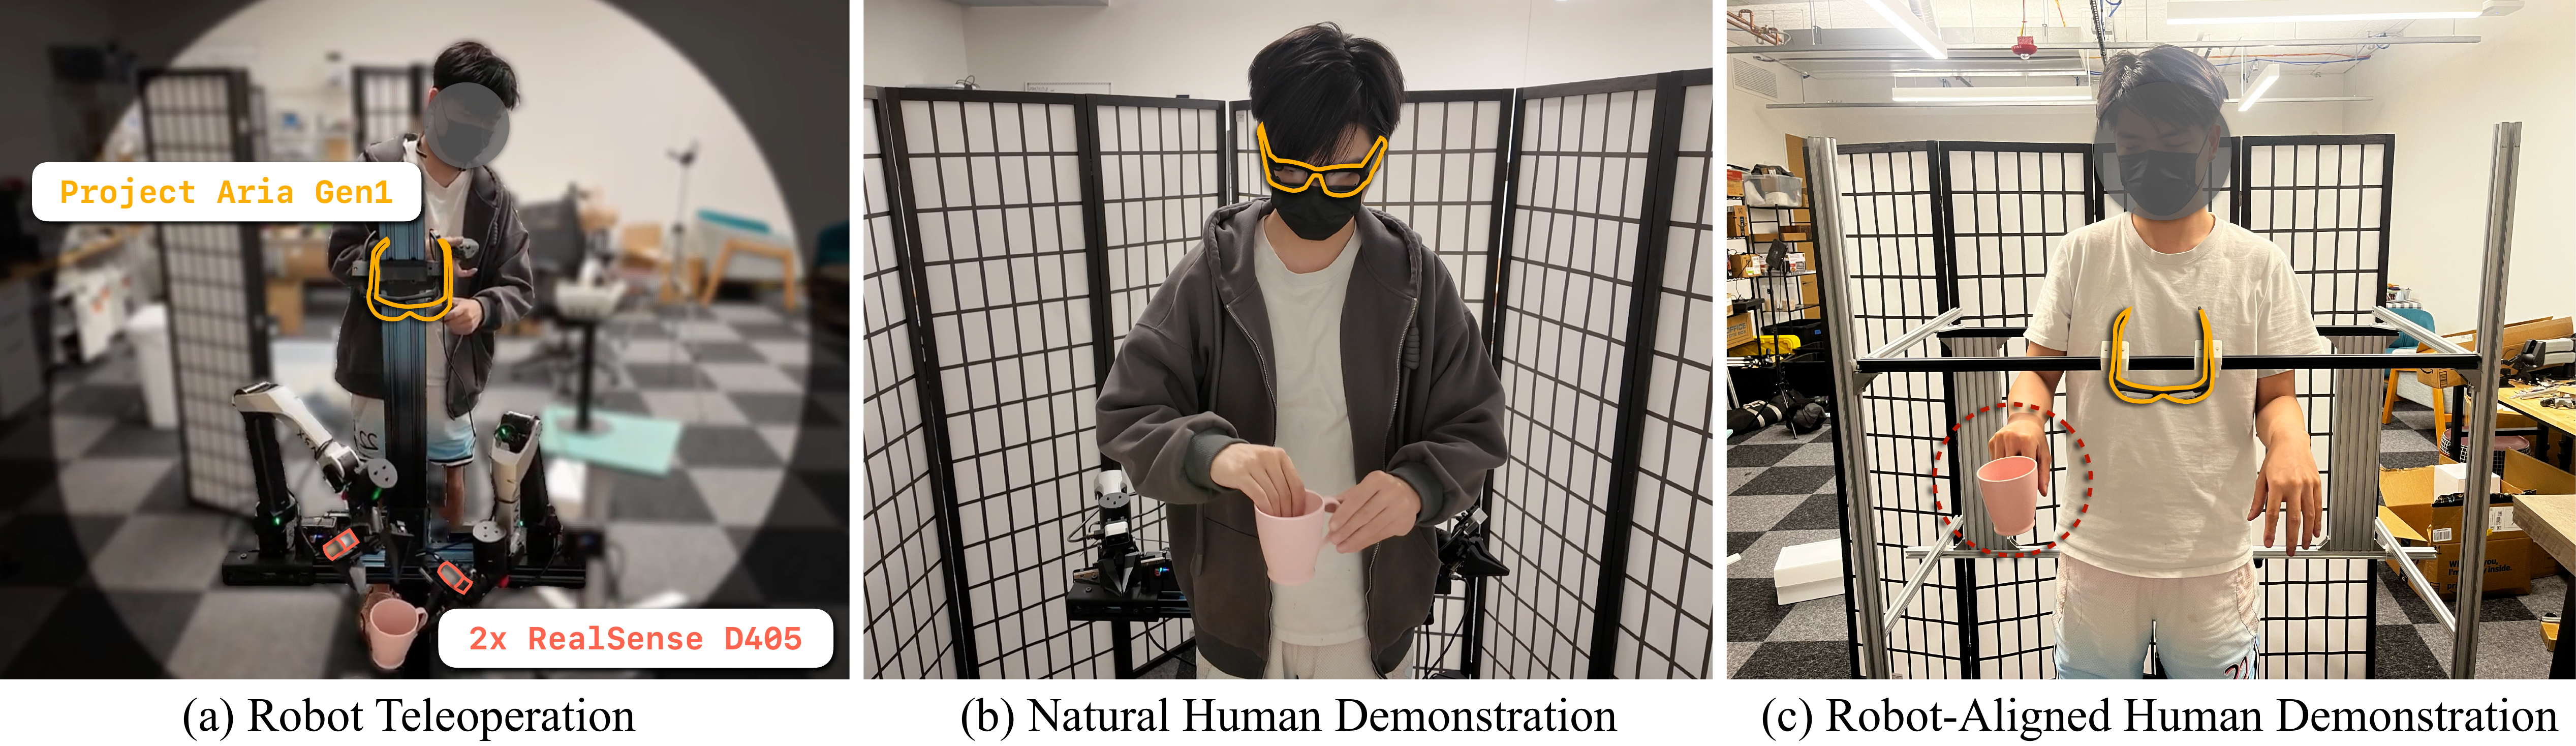}
    \vspace{-16pt}
    \caption{\small
    \textbf{Robot Platform and Data Collection.}
    \textbf{(a)} Our robot platform: two upright-mounted 6-DoF ARX5 arms with two wrist-mounted Intel RealSense D405 cameras and a head-mounted Project Aria headset, teleoperated by a human via a Meta Quest 3 interface.
    \textbf{(b)} A human wearing Project Aria glasses collects demonstrations naturally.
    \textbf{(c)} The human deliberately aligns with the robot's action, height, and viewpoint, producing a static egocentric view matched to the robot platform.
    }
    \label{fig:exp-setup}
    \vspace{-12pt}
\end{figure*}

\suppsubsection{Ablation on Human Data Modality}
\label{supp:subsec:ablation-human-modality}

\begin{wrapfigure}{r}{0.50\textwidth}
\vspace{-40pt}
\centering
\includegraphics[width=\linewidth]{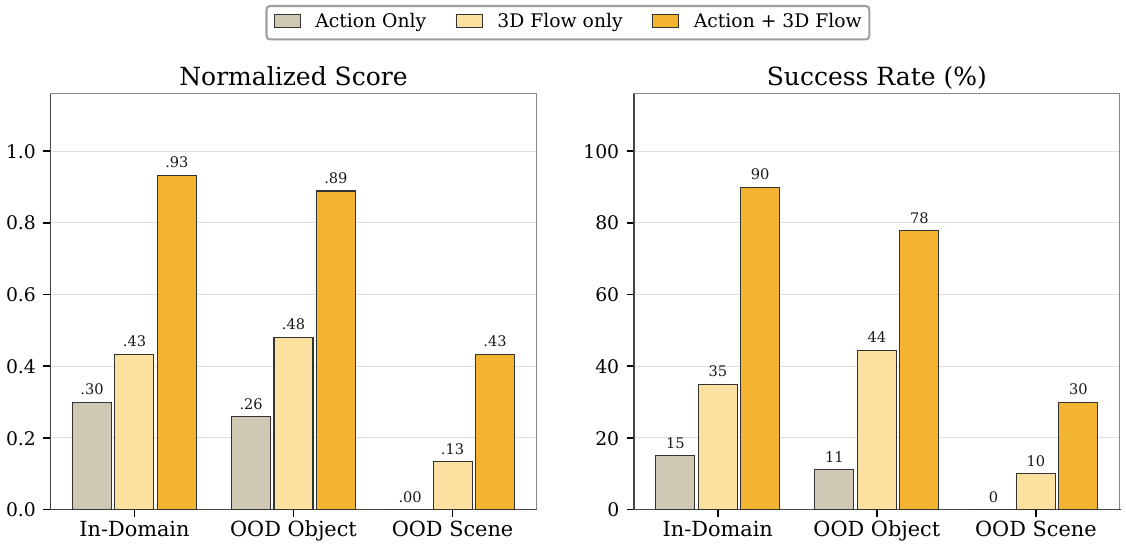}

\vspace{-10pt}
\caption{\small \textbf{Ablation of Co-Train Human Data Modality.} }
\label{fig:exp-ablation-human-modality}
\vspace{-10pt}

\end{wrapfigure}

How much of \egowam's gain comes from the \emph{action labels} on human demonstrations versus the \emph{world-model supervision}? 
We ablate three human co-training modalities on \texttt{cup-on-saucer}: \textbf{Action Only} (BC co-train baseline), \textbf{3D Flow only} (no action supervision on human batches), and \textbf{Action + 3D Flow} (full \egowam).
Fig.~\ref{fig:exp-ablation-human-modality} yields two findings:
\begin{itemize}[leftmargin=*,topsep=0pt,itemsep=0pt,parsep=0pt]
    \item \textbf{World-model supervision alone outperforms action supervision alone.} 
    3D-flow-only outperforms action-only across all three splits, most starkly on OOD~Scene, where action-only fails entirely ($0\%$) while 3D-flow-only retains $10\%$ SR. The trunk shaping induced by predicting 3D motion in human video is a stronger context-level transfer signal than action labels. 
    \item \textbf{Action labels and world-model supervision are mutually reinforcing.}
    Joint training wins on every split, and we attribute this to two complementary effects. (1) \textit{Action as context}: action labels condition the trunk on the demonstrator's intent, sharpening the world model prediction; this effect is measurable directly in the world-model loss, where co-training lowers the 3D-flow prediction loss on both the human and robot streams (Table~\ref{tab:flow_loss_modality}). (2) \textit{Action as task-relevance signal}: action labels mark which motion in the scene is task-relevant, focusing the trunk on agent-caused dynamics rather than incidental flow.
\end{itemize}
\begin{table}[h]
\centering
\caption{3D-flow world-model prediction loss. Adding action labels (\textit{Action + Flow}, full \egowam) lowers the loss over \textit{Flow-Only} on both streams, supporting \emph{action as context}.}
\label{tab:flow_loss_modality}
\begin{tabular}{lcc}
\toprule
\textbf{Flow stream} & \textbf{Flow-Only} & \textbf{Action + Flow} \\
\midrule
Human & $0.23$ & $\mathbf{0.22}$ \\
Robot & $0.20$ & $\mathbf{0.19}$ \\
\bottomrule
\end{tabular}
\end{table}

\suppsubsection{Failure Analysis for Pixel-PT on Bag-Grocery}
As shown in Fig.~\ref{fig:exp-main}, Pixel-PT (robot only) underperforms both BC and Pixel on \texttt{bag-grocery} task. Here, we provide further failure analysis on it. From our observation, most failures occurred at the bag-opening stage, and Fig.~\ref{fig:failure-pt} isolates the cause.
\textbf{Pixel-PT} renders crisp future frames in which the bag already appears open before the gripper has acted on the handles: the natural-image prior, in which bags are typically open, overrides the actual scene state, and the policy advances to the pick stage prematurely.
\textbf{Pixel (from-scratch)} produces blurrier frames but tracks bag openness faithfully, and the resulting policy opens the bag more reliably.
\textbf{Pixel-PT + EgoVerse} keeps the sharp pretrained output while predicting the closed-then-opening progression correctly, indicating that human co-training can correct noisy prior-induced hallucination in pretrained video models by increasing the data amount, and thus improves the policy a lot.
\begin{figure}
    \centering
    \includegraphics[width=\textwidth]{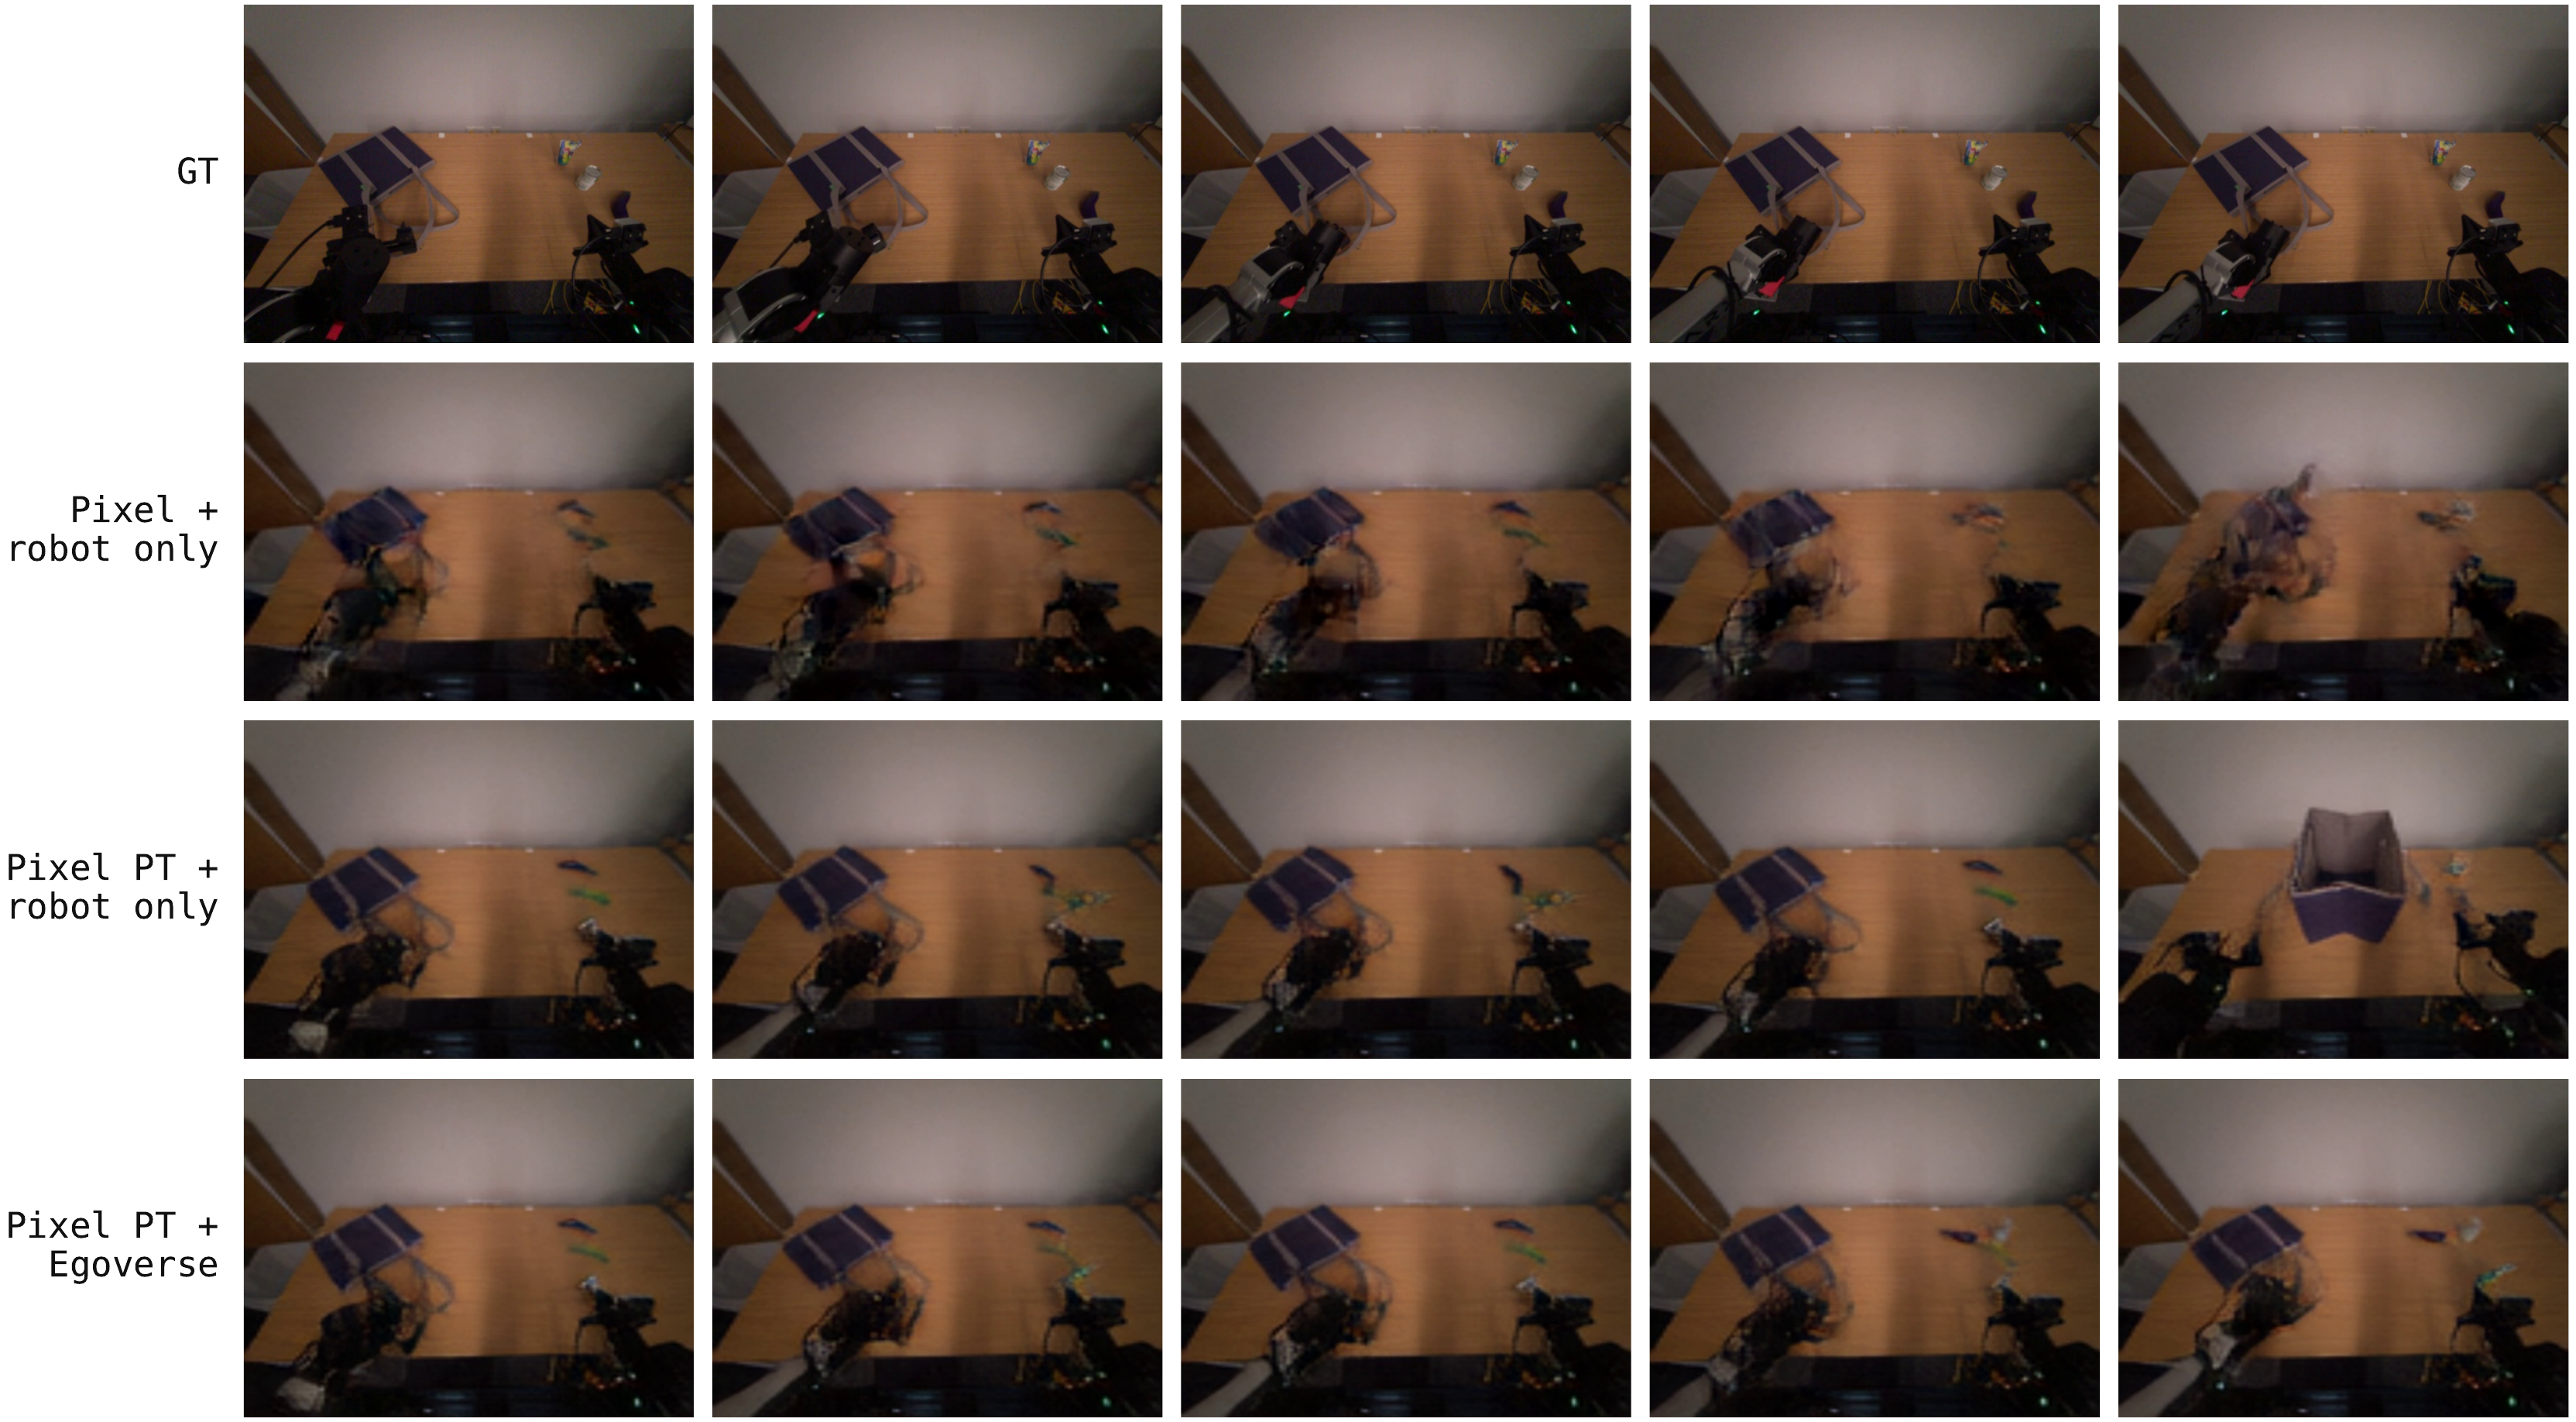}
    \vspace{-18pt}
    \caption{\small
    \textbf{Video Prediction for Failure Analysis on Bag-Grocery.}
    6-step rollouts from the same initial frame. \textbf{Pixel + robot only}: blurry but faithful, where the bag stays closed until acted on. \textbf{Pixel-PT + robot only}: hallucinates an already-open bag, causing the policy to skip the opening stage. \textbf{Pixel-PT + Egoverse}: sharp and faithful, showing human co-training removes the hallucination.
    }
    \label{fig:failure-pt}
\end{figure}
