# Supplementary material for: EgoWAM: World Action Models Beyond Pixels with In-the-Wild Egocentric Human Data
Source: arXiv:2607.08436 source file (2026-10-13)
Supplement: Supplementary file 6 [file 004_robotwin_sim.tex]

\suppsection{Robot-to-Robot Transfer in Simulation: RoboTwin}
\label{supp:sec:sim}

Our real-world experiments (Sec.~\ref{sec:experiments}) establish \egowam's two central claims: that
cross-embodiment co-training transfers across the human--robot gap, and that the world-model head is
the interface that drives this transfer. To validate the same claims in a \emph{public, reproducible,
robot-to-robot} setting, we instantiate \egowam on the RoboTwin~2.0 bimanual
benchmark~\cite{chen2025robotwin2}, which ships teleoperated demonstrations for multiple robots on the
same tasks. The goal here is not a new benchmark result but a controlled replication: under a shared,
dimension-invariant end-effector action space, does cross-embodiment co-training still beat
single-embodiment training, and does the world-model head still help to transfer with abstraction?

\suppsubsection{Simulation Setup}
\label{supp:subsec:rt-setup}
RoboTwin~2.0 runs on SAPIEN~\cite{xiang2020sapien}. We use the bimanual \texttt{aloha-agilex} (two
$6$-DoF arms) as the primary embodiment and \texttt{arx-x5}, \texttt{franka}, \texttt{ur5} as
co-training embodiments, where \texttt{franka} and \texttt{ur5} are two $7$-DoF arms, on three hard tasks: \texttt{pick-diverse-bottles} ($15$-instance bottle pool),
\texttt{stack-bowls-three} (long-horizon manipulation), and \texttt{hanging-mug} (fine-grained manipulation). Each uses the shipped \texttt{demo\_clean-50}
split.

\suppsubsection{Integration and Baselines}
\label{supp:subsec:rt-integration}
We add each robot to the tokenizer stack, reusing the trunk and action head. Because the arms differ
in DoF, we predict for both arms an absolute end-effector action in a head-camera frame---
$[\mathbf{p}_{xyz},\boldsymbol{\theta}_{\text{ZYX}},g]$ per arm ($14$-D)---identical across robots, so
a single action head serves every embodiment and cross-embodiment co-training is well-posed, exactly
as in our real-world formulation (Sec.~\ref{subsec:aligned-action}). At test time the predicted chunk
is resampled to the control rate and streamed to a differential-IK controller~\cite{zakka2025mink}
under a receding horizon. Per task we train every world-model variant \emph{single}
(\texttt{aloha-agilex} only) and \emph{cross} (all four robots), holding trunk, head, and optimizer
fixed. As same-action-space references we adapt RoboTwin's official ACT~\cite{zhao2023act} and
Diffusion~Policy~\cite{chi2023diffusion} pipelines to our setting (\textbf{ACT-EE} and
\textbf{DP-EE}) by replacing their native joint-space state and action with the same $14$-D EE vector
and evaluating through the identical IK executor; they are single-embodiment and world-model-free, so
they isolate what cross-embodiment co-training and the world head add on top of the action space
alone. We evaluate all methods on $100$ held-out seeds ($\geq\!10^5$, sparse success, identical across
methods).

\suppsubsection{Results and Analysis}
\label{supp:subsec:rt-results}

\begin{table}[h]
\centering
\caption{RoboTwin held-out closed-loop success (\%, $100$ seeds). \textbf{Left:} same-action-space,
single-embodiment references (ACT-EE, DP-EE). \textbf{Right:} \egowam variants, each trained single
(\emph{s}) and cross-embodiment (\emph{c}), sharing the trunk and end-effector action head and
differing only in the world target. Best per task in \textbf{bold}. $^{\dagger}$\texttt{stack} is
evaluated on an appearance-shifted object (see text).}
\label{tab:robotwin_variants}
\setlength{\tabcolsep}{4.5pt}
\begin{tabular}{lcc@{\hskip 1.2em}cccccccc}
\toprule
& \multicolumn{2}{c}{\textbf{Baselines}} & \multicolumn{2}{c}{\textbf{BC}} &
\multicolumn{2}{c}{\textbf{Pixel}} & \multicolumn{2}{c}{\textbf{DINO}} & \multicolumn{2}{c}{\textbf{3D~Flow}} \\
\cmidrule(lr){2-3}\cmidrule(lr){4-5}\cmidrule(lr){6-7}\cmidrule(lr){8-9}\cmidrule(lr){10-11}
\textbf{Task} & ACT-EE & DP-EE & s & c & s & c & s & c & s & c \\
\midrule
\texttt{pick-diverse-bottles}          & $2$ & $5$ & $2$ & $6$ & $7$ & $11$ & $4$ & $\mathbf{28}$ & $0$ & $16$ \\
\texttt{stack-bowls-three}$^{\dagger}$  & $0$ & $0$ & $0$ & $0$ & $0$ & $0$  & $0$ & $8$  & $0$ & $\mathbf{16}$ \\
\texttt{hanging-mug}                   & $0$ & $0$ & $0$ & $0$ & $0$ & $\mathbf{1}$  & $0$ & $0$  & $0$ & $0$ \\
\bottomrule
\end{tabular}
\end{table}

Table~\ref{tab:robotwin_variants} reproduces the main paper's findings in robot-to-robot simulation.
Four points stand out:
\begin{itemize}[leftmargin=*,topsep=0pt,itemsep=0pt,parsep=0pt]
    \item \textbf{Cross-embodiment co-training beats single-embodiment training.}
    Every \egowam variant improves from single to cross (DINO $4\!\to\!28$, Pixel $7\!\to\!11$,
    BC $2\!\to\!6$ on \texttt{pick}), and cross is the \emph{only} setting that succeeds at all on
    \texttt{stack}. Since single-embodiment policies already overfit their training scenes yet barely generalize, the gap is genuine cross-embodiment transfer
    rather than better fitting, the same mechanism as our real-world results
    (Sec.~\ref{sec:experiments}).
    \item \textbf{The world-model head, not the action space, drives the transfer.}
    Under cross-embodiment training the world-model variants (Pixel/DINO/3D~Flow) consistently exceed
    the action-only BC policy. The same-action-space but world-model-free references ACT-EE/DP-EE stay
    at or below the single-embodiment variants ($\leq\!5\%$ on \texttt{pick}, $0\%$ elsewhere); since
    they change only the policy architecture, the gain is attributable to co-training through the
    world-model interface.
    \item \textbf{DINO and 3D~Flow are strong at object generalization on the first two tasks.}
    Both \texttt{pick} and \texttt{stack} stress object generalization, and the appearance-abstracting
    targets lead. On \texttt{pick} (a $15$-instance bottle pool) DINO reaches the best $28\%$ and
    3D~Flow $16\%$. On \texttt{stack}, an incidental asset change between the released demonstrations and
    the current simulator (the bowl's material shifted while its pose and geometry did not, and
    \texttt{demo\_clean} adds no texture randomization) turns evaluation into an appearance-shift test;
    \emph{only} the appearance-invariant DINO ($8\%$) and 3D~Flow ($16\%$) survive it while BC and Pixel
    collapse to $0\%$, directly reflecting the appearance-abstraction criterion~(D1) of
    Sec.~\ref{subsec:world-variants}. 
    \item \textbf{Very fine-grained manipulation still fails for all methods.}
    \texttt{hanging-mug} requires threading a mug onto a thin rack (a millimeter-precise insertion) and
    here \emph{every} method, including DINO and 3D~Flow, stays at $\leq\!1\%$. The bottleneck on this
    task is manipulation precision, not object generalization or the world target: the appearance
    abstraction that carries \texttt{pick} and \texttt{stack} does not by itself supply the
    sub-centimeter accuracy this insertion demands. Closing this gap is orthogonal to the transfer gains
    above and is left to future work.
\end{itemize}
